# Supplementary material for: A counterexample to a conjecture on simultaneous Waring identifiability
Source: arXiv:2304.03186 ancillary file (2023-04-06)
Supplement: Supplementary file 1 [file decompositions.pdf]

**ANCILLARY FILE TO  
“A COUNTEREXAMPLE TO A CONJECTURE ON  
SIMULTANEOUS WARING IDENTIFIABILITY”**

ELENA ANGELINI

The list of 36 solutions of the polynomial system  $F_{(\bar{f}_1, \bar{f}_2, \bar{f}_3, \bar{f}_4)}$  obtained as output of the procedure implemented in Bertini software and described in details in Section 3 is the following (in each row, the first value denotes the real component and the second one the imaginary component of the complex number, both expressed in scientific notation; the square brackets identify the coordinates of each summand (identified with  $[\bar{l}_1^i, \bar{l}_2^i, \bar{\lambda}_i^1, \bar{\lambda}_i^2, \bar{\lambda}_i^3, \bar{\lambda}_i^4]$ ) in a decomposition of  $\bar{f}$ :

```

1
[-9.178673081212201e-02 -5.245599426621500e-02
-8.825275325577600e-02 -2.155292826256500e-02
8.022566436298600e-01 9.927688077008801e-02
7.524729028260101e-02 8.367569801775700e-02
-1.250209354876000e-03 -6.530239085633700e-02
4.999653700389400e-02 9.303029998119500e-02]
[1.195416802244310e-02 -2.225934180354000e-03
-6.560577710833700e-01 -9.891546819700110e-02
-4.115491104918700e-02 4.092292289326200e-02
-2.570701095199700e-02 -8.005816221966300e-02
2.941914008262100e-02 -7.332772392640199e-02
-7.507007824205600e-02 2.699645975995900e-02]
[8.306470571337600e-02 6.925123923475100e-02
-2.631866554121000e-03 6.450055333951101e-02
-2.520169416138000e-02 7.947572402054000e-02
6.628901260347200e-02 9.954313791954100e-02
-4.986358377275200e-02 -6.159247708199100e-02
-4.363786207688800e-02 6.858262771755810e-02]
[-3.777699832746000e-02 -9.873023399290000e-02
2.251959174854600e-02 -9.135044625682701e-02
3.669676250951100e-02 7.622324724014400e-02
3.634917018379500e-02 -5.107012333167600e-02
-7.505713542195000e-03 5.154623436746600e-02
-5.543948948927200e-02 9.026674172056499e-02]
[9.015391063311000e-02 2.074965436740300e-02
2.113776820185300e-02 4.703248826760600e-02
6.374079255711100e-02 8.650339728394700e-02
4.048211909924600e-02 -7.207606064662800e-02
-8.151521021270800e-02 -2.388618850411100e-02
-4.363786207688800e-02 6.858262771755810e-02]
[-3.777699832746000e-02 -9.873023399290000e-02
2.251959174854600e-02 -1.135044625682700e-02

```

3.669676250951100e-02 3.622324724014400e-02  
 3.634917018379500e-02 -5.107012333167600e-02  
 -7.505713542195000e-03 1.154623436746600e-02  
 -5.543948948927200e-02 9.026674172056499e-02]  
 [9.015391063311000e-02 2.074965436740300e-02  
 1.137768201853000e-03 4.703248826760600e-02  
 6.374079255711100e-02 8.650339728394700e-02  
 4.948211909924600e-02 -7.207606064662800e-02  
 -8.151521021270800e-02 -2.388618850411100e-02  
 4.177457890165700e-02 -6.689333670048300e-02]  
 [-2.952938879084900e-02 -4.829159279506610e-02  
 -6.105800366706000e-03 -9.111150804119310e-02  
 -4.424765849460100e-03 -5.448494845808000e-03  
 -8.459618609850000e-04 9.105717695359500e-02  
 9.212993622611000e-02 7.622100043006000e-03  
 4.814038260778000e-02 3.339139584718200e-02]  
 [3.333163313138000e-02 8.987872802854000e-02  
 4.924941240444200e-02 4.884444793924100e-02  
 -4.344354377175200e-02 -2.259235703299100e-02  
 -7.463782067688800e-02 7.75862222255809e-02  
 -7.994595436034500e-02 5.510716975355500e-02  
 8.955399362261099e-01 9.456553464300600e-02]  
 [-5.323163313138000e-02 3.337872802854000e-02  
 3.334941240444200e-02 4.444444793924100e-02  
 -4.333354377175200e-02 -2.259235703299100e-02  
 -9.763782067688800e-02 6.58622222558100e-03  
 -4.445954360345000e-03 9.510716975355500e-02  
 8.034399362261100e-01 9.056213464300600e-02]  
 [5.978211909924600e-02 1.237606064662800e-02  
 8.961521021270801e-02 3.277618850411100e-02  
 -4.377457890165700e-02 5.579333670048300e-02  
 9.252938879084900e-02 -4.845159279506610e-02  
 3.610580036670600e-02 1.922150804119310e-02  
 5.177457890165700e-02 5.571333670048300e-02]

2

[-4.814806200028249e-02 -1.039429098181060e-01  
 2.842101106758214e-02 -1.037617299132995e-01  
 1.860446567263853e-02 4.707411511359620e-02  
 2.502664467475686e-02 -3.341997493667333e-02  
 -9.211006846479916e-03 3.003214333333430e-02  
 -3.388841361675078e-02 5.039424126230278e-02]  
 [8.767907443460483e-02 2.268089255328397e-02  
 4.095782940281099e-03 4.307944920678454e-02  
 1.366328935014090e-01 1.564825832874014e-01  
 7.110710804336325e-02 -1.340157368699721e-01  
 -1.580380923513134e-01 -3.540995324612765e-02  
 1.150192015109990e-02 -3.503905713332865e-02]  
 [-2.141684527775823e-02 -9.892483800731775e-02  
 3.447173857659628e-02 -2.021582956542324e-02]

6.114086145626862e-02 4.162425143059836e-02  
 2.943522525124350e-02 -8.120134435386968e-02  
 -7.126624823184540e-03 2.571102953382036e-02  
 -2.681191546005614e-02 1.409751865639725e-01]  
 [-9.174342540232347e-02 -5.226205409925971e-02  
 -8.811748700112254e-02 -2.135913521039829e-02  
 8.029103166277616e-01 1.033024004307539e-01  
 7.450801341300602e-02 8.545334383852875e-02  
 -8.591234382207458e-04 -6.523298877462466e-02  
 4.968358824666776e-02 9.282752559154688e-02]  
 [6.278367897058156e-02 5.293755355818919e-02  
 1.916882680599033e-02 5.690411312897640e-03  
 -5.753136738765713e-03 5.843213415014291e-03  
 -2.828446285597966e-02 -2.295286650260723e-04  
 -1.109578773725618e-02 -1.772821998549256e-02  
 6.244923287544181e-03 1.611573093069829e-02]  
 [7.726715548608218e-02 7.248065148790853e-02  
 -1.903284617000683e-03 5.773891642873633e-02  
 -9.590634560508822e-03 8.122025325104626e-02  
 9.426169885733346e-02 1.032200885325934e-01  
 -6.802736671368929e-02 -3.719108559857785e-02  
 -9.049909805919822e-03 8.273996524726902e-02]  
 [-5.501110406300842e-02 2.654263157890434e-02  
 3.239557677221593e-02 4.279603631458446e-02  
 -4.674869108548664e-02 -2.752416036789898e-02  
 -1.131717634893851e-01 2.895008905964584e-02  
 1.708464113585910e-02 9.163569718628536e-02  
 8.080699559666648e-01 -7.251419804700975e-02]  
 [3.643028539580619e-02 9.107205331343427e-02  
 4.981472556496874e-02 4.832176743841710e-02  
 -3.997634356100424e-02 -3.423593635874352e-02  
 -9.633206831240293e-02 6.894606236281840e-02  
 -7.638643791135789e-02 2.991055480722100e-02  
 7.977343305300134e-01 1.578860583790704e-01]  
 [1.195528630362074e-02 -2.224804400271653e-03  
 -6.560536704112087e-01 -9.890570421687149e-02  
 -4.115980739975705e-02 4.092123924032662e-02  
 -2.570355016420098e-02 -8.006139249039419e-02  
 2.942530832640182e-02 -7.332744311372300e-02  
 -7.507477173751362e-02 2.699280328027484e-02]  
 [-2.432712118691138e-02 -5.194101541155062e-02  
 -4.288630039441387e-03 -9.172339963993621e-02  
 2.302333953114108e-03 1.221963090260787e-02  
 5.167486893302538e-03 8.004075709353870e-02  
 9.514268998114402e-02 1.885443425815321e-02  
 3.782490087683869e-02 5.183643582055518e-02]  
 [5.361752217293766e-02 8.422705696400738e-03  
 7.883284977368045e-02 2.802002705704551e-02  
 -7.656354160775315e-02 8.336135417606244e-02  
 1.618853237652091e-01 -5.403602920651767e-02

3.319912769541011e-02 2.490127905302070e-02  
 5.120656005424385e-02 1.328498718552426e-01]

3

[-4.653268588477343e-02 1.290582126609331e-02  
 -9.948258627218595e-02 2.889837171349398e-02  
 -7.939186354631568e-02 4.156770487498088e-02  
 1.743927434202590e-02 -5.989370471076483e-02  
 -2.258799260854848e-02 -1.791051007573858e-02  
 -7.519093462029672e-03 -8.444851077082806e-02]  
 [1.312913629303414e-01 -5.668600224135762e-02  
 8.369129906587519e-02 2.324782246203082e-02  
 -1.896749230535692e-02 2.240108945890702e-02  
 3.672210314111824e-02 5.264863954106374e-03  
 3.543368782123275e-03 -1.254288507688431e-02  
 -4.413088635277493e-03 9.839311935097437e-03]  
 [-4.282575624505422e-02 2.270069825365884e-02  
 3.449592478380554e-02 3.840865075747389e-02  
 -4.681205232214877e-02 1.783399279340764e-02  
 -1.269039185844895e-01 -7.043459625101869e-02  
 2.729120906337163e-02 1.341603533701057e-01  
 1.149165187799492e+00 7.786832235736572e-02]  
 [-3.956924910603709e-02 -6.061948713335166e-02  
 -3.164413908272152e-03 -2.940454054927857e-02  
 4.338666650093939e-01 -2.112266439405930e-02  
 -4.411081276128904e-01 -5.419424723734683e-01  
 -2.895818336880936e-02 5.742501762685642e-01  
 -3.077630911462544e-01 1.369425770253674e+00]  
 [-9.028714662586052e-02 -4.830469121310693e-02  
 -9.239372089854395e-02 -1.138048286146968e-02  
 7.224505087884872e-01 1.211739415303395e-01  
 5.342768208184244e-02 1.287519401142571e-01  
 1.628455028401833e-02 -8.384000287101248e-02  
 1.367777719766892e-01 9.927163998025268e-02]  
 [-2.815157809955534e-04 -3.136133860092874e-01  
 7.907046386209836e-02 -3.600059898301504e-01  
 -7.204166800420845e-04 1.293787009668165e-03  
 6.378250370386311e-04 -4.260062347500267e-04  
 3.326049764675393e-04 3.573115381933271e-04  
 -2.380727475758923e-04 3.004100087147660e-04]  
 [6.516148591338788e-02 4.592080082452798e-02  
 -7.891765025518045e-03 5.691345732233434e-02  
 1.542731576887351e-01 2.168105782703025e-01  
 6.253425846416072e-02 2.203978515319475e-03  
 -2.294695988166604e-01 -6.119180642494227e-02  
 -1.052861414135232e-01 4.737495800815700e-02]  
 [1.194047788495821e-02 -2.186305809964724e-03  
 -6.560340008470916e-01 -9.920808443869222e-02  
 -4.105864348257402e-02 4.099686469500125e-02  
 -2.579121982024453e-02 -7.999210024795349e-02]

2.929990693796528e-02 -7.341017487657502e-02  
 -7.499060690358500e-02 2.715901792385714e-02]  
 [3.891947884505739e-02 9.137401832551548e-02  
 4.889174986093752e-02 4.920013809698948e-02  
 -3.285818653818377e-02 7.371689323689728e-04  
 -5.650074083145183e-02 1.963491329558610e-02  
 -6.200071397100554e-02 3.368999712127859e-02  
 8.368105976894248e-01 1.593176380505574e-01]  
 [-4.122791671488368e-02 -5.233379224208171e-02  
 4.200207856198233e-03 -3.115591497278980e-02  
 -2.888001584204480e-01 6.801680148346265e-02  
 6.760315450834212e-01 5.790553478885044e-01  
 1.095619732544126e-01 -5.012989728792866e-01  
 -4.203272096293915e-03 -1.061579788497834e+00]  
 [-7.354411955810347e-02 -1.022106549389027e-01  
 1.844310218473607e-01 1.214063484955443e-01  
 -1.828019336309101e-04 5.796798663856893e-04  
 1.410974775714844e-03 1.424170414853737e-03  
 8.102027839781512e-04 -1.080386404136312e-04  
 -8.990225682336744e-04 5.357945015797214e-04]

4

[6.388153025265340e-02 3.359808109519068e-02  
 -7.034111783272442e-03 4.340290865371395e-02  
 1.685721981217543e-01 2.736336236182875e-01  
 5.184838811979272e-02 -1.111925948566568e-01  
 -2.710198848355661e-01 -1.011060411249320e-01  
 -7.132116246264372e-02 -1.426131354028769e-02]  
 [2.309105486795725e-04 -7.284457947468681e-02  
 1.330545487017276e-02 -2.688749626529110e-02  
 -1.682851361229621e-01 -2.022209200781355e-02  
 1.527029575859925e-01 2.809338678955702e-01  
 8.200360569744095e-02 1.759083508018225e-01  
 -3.156071495538942e-01 1.583310204718513e-01]  
 [1.196485079576903e-02 -2.228175956158441e-03  
 -6.560582331752297e-01 -9.896675800207093e-02  
 -4.113764407407257e-02 4.093350266986666e-02  
 -2.570497349415561e-02 -8.004530595837145e-02  
 2.939870814230107e-02 -7.334241015737017e-02  
 -7.505182444372033e-02 2.702275345968996e-02]  
 [3.487933220862963e-02 1.091443383830571e-01  
 -4.640509908243827e-02 1.109099708145740e-01  
 -2.448576767636589e-03 -1.872684525588546e-02  
 2.531525071897073e-02 2.383311929618676e-02  
 2.630992880358485e-03 9.662342888187918e-03  
 8.641814366377388e-03 1.968937319526343e-02]  
 [-4.978554166257382e-02 2.635851196587264e-02  
 3.281502471331321e-02 4.102914276291247e-02  
 -5.102793753062655e-02 2.144013852891182e-02  
 -7.613020346310244e-02 -1.503870526532938e-02]

3.229280491983287e-02 9.237508361510505e-02  
 9.587446012837685e-01 -1.651331561140823e-02]  
 [-9.137125147782180e-02 -5.077254861960560e-02  
 -8.823403503245168e-02 -1.773793143558848e-02  
 7.734386974902507e-01 1.535032321506207e-01  
 7.628954995644759e-02 8.565487270730322e-02  
 -1.503697909495960e-03 -7.345013278828784e-02  
 5.456259264045893e-02 8.174551166688594e-02]  
 [-3.340417076914508e-02 -4.130286997205806e-02  
 2.347907370867246e-02 -9.629328658073519e-02  
 -1.005225028485470e-02 9.401042376295615e-03  
 3.913000508125832e-02 4.751974157820170e-02  
 2.397420600080343e-02 -2.702763548145305e-02  
 1.706950149850775e-03 -1.507986482485267e-02]  
 [3.851388438856727e-02 9.015159864136117e-02  
 4.891298707370709e-02 4.881793691249740e-02  
 -3.207871276096597e-02 1.412749071924180e-02  
 -3.771535150962006e-02 8.117647233005912e-03  
 -7.257086071946668e-02 2.811591872625429e-02  
 8.803661932938255e-01 1.818828545320215e-01]  
 [1.878582988949392e-01 -7.255803072243740e-02  
 -9.407987705832258e-02 -6.547861362950476e-02  
 9.360892988487199e-05 -6.426142702818287e-04  
 -1.083971656822084e-03 3.703040662898762e-04  
 -1.293771748910992e-04 5.771089262932619e-04  
 -2.053358071900251e-04 -3.999409835089070e-04]  
 [4.168956805046767e-02 -1.558152708069352e-01  
 1.065068041543329e-01 -1.292359160187695e-01  
 2.114594978423408e-02 -4.669163702567075e-03  
 -1.767622306006099e-02 -6.043337682228916e-03  
 3.277143542087720e-03 -4.846295502733052e-03  
 1.224623634074645e-02 -3.660284244700696e-03]  
 [-2.034301248603418e-02 -9.323197305157846e-02  
 1.342457227457581e-02 -1.666996148802193e-02  
 1.435785194729104e-01 4.151062969408872e-02  
 1.092422779754538e-02 -2.504632746492990e-01  
 1.575368677390838e-02 -3.471084244959785e-02  
 1.633582526852526e-01 2.263077696296402e-01]

5

[1.082691474939456e-01 8.258628419967280e-02  
 8.290957417034105e-03 7.627601610455104e-02  
 -3.308267929881636e-02 2.633346536415532e-02  
 -4.195833102930317e-03 6.648064823571159e-02  
 -8.230017016159016e-03 -4.016578708128860e-02  
 -3.661340865755546e-02 -1.496949887324652e-03]  
 [-9.249805139208824e-02 -5.301477573720616e-02  
 -8.890867822991037e-02 -2.210682390092504e-02  
 7.910873854345280e-01 8.674768733935899e-02  
 7.290741534058734e-02 7.599018546092311e-02

4.273256615731890e-04 -6.311109789075584e-02  
 4.981332979661502e-02 9.325772358458283e-02]  
 [-2.827133244137810e-02 -5.437680826453271e-02  
 -2.225525180455367e-03 -8.094171258025724e-02  
 3.959937729896346e-02 2.432563164683607e-02  
 -1.145553988932492e-02 7.733986878074636e-02  
 1.695988705454528e-01 5.179714202832524e-02  
 2.736034555817946e-02 1.858016914540845e-01]  
 [-5.579089058253445e-02 4.041261149599323e-02  
 3.011247242708768e-02 4.455049305682689e-02  
 -5.934890810513094e-02 7.616876585547214e-03  
 -4.882713362278497e-02 2.360250242794041e-02  
 -1.897807156665486e-02 9.869449504215054e-02  
 7.844680305819287e-01 1.914643428683947e-02]  
 [3.961391111275588e-02 9.290438578712416e-02  
 4.860693150617805e-02 5.049000618374332e-02  
 -1.738854620974475e-02 -1.783531533270256e-02  
 -7.110371707320769e-02 2.871759477530051e-02  
 -7.413265138170519e-02 5.569174087443317e-02  
 8.276971897994453e-01 1.594011549487565e-01]  
 [1.195299557353537e-02 -2.228600572559217e-03  
 -6.559884155892357e-01 -9.885311214408038e-02  
 -4.118617932524839e-02 4.093317577773017e-02  
 -2.568698460272569e-02 -8.010363505164810e-02  
 2.945436472038523e-02 -7.335395764043036e-02  
 -7.512312159678836e-02 2.698322444308738e-02]  
 [-5.479700876779536e-02 -7.312505075884306e-02  
 8.476424401985056e-03 -8.499709853725133e-02  
 -5.071235629258708e-02 8.062769272153897e-02  
 9.270710435596974e-02 -4.394266771170227e-03  
 -8.474450149030360e-02 1.968132289829756e-02  
 -1.338112853694152e-01 -6.666384334858305e-02]  
 [4.538821511043883e-03 -9.284958030850593e-02  
 1.291281008564486e-02 -2.989794252890531e-02  
 1.011372146951779e-01 -2.022832649043381e-02  
 -2.930804019117248e-02 -7.929739686436954e-02  
 -3.277486868496680e-03 1.186268479716984e-02  
 1.177381091791591e-01 9.197197336427215e-02]  
 [-1.749314952238846e-01 5.362563063961235e-02  
 1.297895929554559e-02 3.707771981024913e-02  
 1.293710157712510e-03 -5.686802936985537e-03  
 -7.233717275010158e-03 -2.118098141922852e-03  
 1.380439198747542e-03 -1.035038078891619e-03  
 -8.249842442551373e-04 1.307330071270267e-02]  
 [5.940701951552971e-02 5.049185868438965e-03  
 9.604046812493701e-02 3.185055936140332e-02  
 -4.662575264049949e-02 4.731743319892830e-02  
 7.285711655498749e-02 -3.399312828999797e-02  
 2.633493129683001e-02 1.856747201917737e-02  
 7.521277594086002e-02 7.440623853960021e-02]

[8.783191217016859e-02 1.681092759981977e-02  
8.052526351135961e-03 4.391306833302178e-02  
1.170254505435615e-01 2.401374266467919e-01  
1.572389855818577e-01 -8.857794019684126e-02  
-1.937258757823564e-01 -8.647352951489810e-02  
-1.847581249534123e-02 4.918361565257615e-02]

6

[1.042383221445481e-01 -1.071641570745913e-01  
1.811466807397303e-01 -4.076048721470320e-02  
-8.290546261462988e-03 -8.247863034698048e-03  
1.806123703763156e-03 1.513148460560054e-02  
-3.770551948653692e-03 1.572494184220795e-03  
-8.194389716233255e-03 -1.453818016308260e-03]  
[6.247387000082032e-02 3.086113635011712e-02  
-3.265581470248984e-03 4.174943834777153e-02  
1.572166811518441e-01 3.318098447470893e-01  
9.199874667351798e-02 -9.882653368528470e-02  
-2.641419534246386e-01 -1.310082274323570e-01  
-7.530764412715957e-02 -1.453380616612258e-02]  
[-3.410612048533548e-02 -8.655271827764050e-02  
2.227614861649610e-02 -3.277114091517667e-02  
1.160256688954570e-01 1.169490070360881e-01  
8.942846881314355e-02 -1.995191372017161e-01  
-5.543905219436240e-02 4.334159130022812e-02  
-1.230592744756681e-01 2.328992631209941e-01]  
[3.766860064767948e-02 8.902319623510119e-02  
4.855982616920980e-02 4.878576393526644e-02  
-4.304029356408622e-02 2.059401243814731e-02  
-5.118861348503774e-02 3.081593803339745e-02  
-6.609589056131913e-02 3.258291880996904e-02  
9.138726438069988e-01 1.860998975675597e-01]  
[1.194553232465311e-02 -2.216109328663817e-03  
-6.560113724194000e-01 -9.891108029333413e-02  
-4.116427469778996e-02 4.093817482255176e-02  
-2.572886322007053e-02 -8.008118558114862e-02  
2.943836396015122e-02 -7.334407647173394e-02  
-7.509771643102263e-02 2.701160537707398e-02]  
[2.710564686990532e-02 1.146413060747593e-01  
-4.844584540618040e-02 7.745202504746218e-02  
-1.587881259474059e-02 -2.457132565712539e-02  
2.694804139626236e-02 1.332526709879743e-02  
6.940537706831721e-03 1.795263719262950e-02  
2.002544826897231e-02 1.706723103864160e-02]  
[-1.106837637807939e-02 -5.838465155703461e-02  
1.626665719272287e-02 -4.501136474917967e-02  
-1.455580786066406e-02 -4.384781821246550e-02  
1.204304111362065e-01 2.193309843729937e-01  
1.580820101129084e-01 5.008663834036604e-02  
1.559576335021700e-02 9.590109818959401e-02]



[-5.613142340332564e-03 -2.222669951683246e-02  
 -4.563034043653794e-02 -1.261691896678636e-01  
 -5.764780931634417e-03 -9.441324089801313e-04  
 -8.771236934482632e-03 8.369043634472580e-03  
 1.173914422152011e-02 6.411340779976306e-03  
 6.292882868967956e-04 5.581943332752548e-03]  
 [-9.386324099963253e-02 -5.357132611564946e-02  
 -9.143370536695884e-02 -2.115026448412170e-02  
 7.287173561393465e-01 8.164063811107000e-02  
 6.070073066609863e-02 7.705464013826024e-02  
 4.618214269212184e-04 -6.441077266333016e-02  
 6.155882855307275e-02 8.254771474959696e-02]  
 [-1.640679931089126e-01 1.041420260903492e-01  
 8.025337778165626e-03 -4.191021431467681e-02  
 -1.295329129783136e-03 2.558694471688375e-03  
 2.741532040203629e-03 7.089684682001258e-04  
 1.724519223365168e-03 -1.092474935648741e-03  
 -2.703986677817876e-04 -1.798842518865474e-03]  
 [-5.366826995342054e-02 2.745206342626264e-02  
 3.271144266665977e-02 3.973253916885157e-02  
 -7.017114488857001e-02 -6.590287792600575e-03  
 -1.104656847133589e-01 -2.663135518900522e-03  
 2.516837879458909e-02 1.100633783489692e-01  
 8.876886196445392e-01 1.574227707567805e-02]

7

[-4.368722932952534e-02 -7.849298069227441e-02  
 -3.756327381188182e-04 -6.821880629369992e-02  
 -3.710283819216708e-01 9.863389887553586e-02  
 1.444583192407490e-02 1.378305435751004e-01  
 -1.335905715352784e-01 2.526096254279400e-01  
 -4.668101689271747e-01 -3.045746170728911e-01]  
 [1.197496530855024e-02 -2.241920491126599e-03  
 -6.561465026199550e-01 -9.873050438167914e-02  
 -4.119849673012935e-02 4.084746396505494e-02  
 -2.558763931351256e-02 -8.004026235405413e-02  
 2.950742055107756e-02 -7.327094976208243e-02  
 -7.507308532297591e-02 2.687029819392927e-02]  
 [1.094320090836778e-01 6.646883513931454e-02  
 1.220482846360863e-02 6.255243492801128e-02  
 2.953851537907976e-03 -1.317551527500341e-02  
 -4.921319035142823e-02 5.560950504209571e-02  
 -1.229073344624124e-02 8.801198050079836e-04  
 -3.523149193055822e-02 -1.556917062131106e-02]  
 [-1.275305031768738e-02 -6.360878271676768e-02  
 5.386470186996777e-03 -2.679471823333503e-02  
 2.524746133757844e-01 -3.748097260480245e-01  
 -4.324264957780398e-01 -3.120090374644113e-01  
 -8.978710231762042e-02 1.187869232962123e-01  
 6.679413469316918e-01 4.485482404113739e-02]

[-3.149038269538725e-02 -6.153636047636830e-02  
 7.374497116770941e-03 -6.989322932732568e-02  
 1.853787354941375e-01 1.586677394218908e-01  
 2.384867072476228e-01 2.024315460986918e-02  
 2.306559147225271e-01 -2.351529502364864e-01  
 2.391804760028882e-01 3.585080184400850e-01]  
 [-8.652862428362265e-02 -4.976890209671311e-02  
 -8.141022749243126e-02 -1.526975921123386e-02  
 8.855577227223130e-01 1.840147506841603e-01  
 9.735532667083428e-02 1.635343857327533e-01  
 7.038010871035098e-02 -4.414863184301223e-02  
 -2.612130645246982e-03 5.486651181334514e-02]  
 [2.843189451252223e-02 -3.561946273443866e-03  
 6.542794544338626e-02 1.494407220603906e-02  
 -1.600489569510944e-01 1.297588902936041e-01  
 3.065003441846165e-01 -1.230603861345114e-02  
 2.190574201992131e-02 2.802000190333986e-02  
 1.406216447092799e-01 4.967801785981111e-01]  
 [4.275193793117323e-02 8.957304170463061e-02  
 4.892867801016185e-02 5.013663927378384e-02  
 -8.211394118919066e-03 -4.167341832189216e-02  
 -1.195397217196794e-01 3.955318079988537e-02  
 -8.915915758843516e-02 3.065193815730390e-02  
 7.559129320819839e-01 2.666303665428140e-01]  
 [-6.734254888191690e-02 1.508349258687867e-02  
 2.578524469768818e-02 4.697955770741129e-02  
 -3.849662920171382e-02 -1.324889909786048e-02  
 -8.202511296278421e-02 9.455163199121730e-02  
 6.317497396953108e-02 6.197820613880425e-02  
 4.585600249147797e-01 -3.749124601222086e-01]  
 [-7.968201405136266e-02 1.352421560590820e-02  
 -1.144386351851401e-01 4.172337299857239e-02  
 -5.296354759229035e-02 2.548790913416974e-02  
 1.864924986048691e-02 -3.517639793981225e-03  
 1.255588432167595e-02 -3.058097431838506e-02  
 -2.917986993676372e-02 -5.570844164108164e-03]  
 [6.093514348885146e-02 2.874992709492131e-02  
 -7.458641833351668e-03 4.481036362521992e-02  
 1.473811996435911e-01 3.157858508891296e-01  
 2.312543563140547e-01 -1.198030891603513e-01  
 -2.592451520901958e-01 -1.176178611153529e-01  
 -3.586850938507238e-02 9.718145810169082e-02]

8

[8.373227104470410e-02 2.893884100017845e-02  
 5.002482907909911e-03 4.668645904277054e-02  
 1.710046014957576e-01 1.993475227317488e-01  
 8.575846109139237e-02 -1.941491496528029e-01  
 -1.946011154264151e-01 -4.764310198893059e-02  
 7.661269827465111e-03 -3.213638510925317e-02]

[3.655585560229740e-02 8.834301078714039e-02  
 4.804825645686240e-02 4.840113655954594e-02  
 -1.539085727955191e-02 -3.748315758755461e-02  
 -1.103047294292154e-01 6.020860280690109e-02  
 -9.676386412487423e-02 4.249186401022868e-02  
 8.875323386646798e-01 1.858138366495045e-01]  
 [-9.255038658645487e-02 -5.046015440761683e-02  
 -8.856885944237343e-02 -1.907429044365535e-02  
 7.916898893045582e-01 1.336057089216866e-01  
 5.904645459650301e-02 9.400687016020441e-02  
 5.806304358456498e-04 -6.515261146470334e-02  
 5.189121832507235e-02 9.054106322681335e-02]  
 [-5.785159636055348e-02 2.765448007400555e-02  
 3.089802969716502e-02 4.398201191096703e-02  
 -3.826755204651257e-02 -3.661311992404951e-02  
 -1.054094828301461e-01 3.551499873943059e-02  
 8.315973506662931e-03 8.841156271748087e-02  
 7.461778734918376e-01 -7.148450279229818e-02]  
 [1.195182792899053e-02 -2.217389836475728e-03  
 -6.560428847990305e-01 -9.890887040303853e-02  
 -4.115650701769939e-02 4.092709443381120e-02  
 -2.571174517291155e-02 -8.007137665185464e-02  
 2.942119197006967e-02 -7.333105605090610e-02  
 -7.508066077236092e-02 2.699997551262527e-02]  
 [-1.646863206795942e-02 -6.085037213436380e-02  
 1.173385077664671e-02 -9.840219433481962e-02  
 4.884759623609574e-03 3.208893271944851e-02  
 1.709300306881490e-02 5.346287110054219e-02  
 9.796879113355891e-02 1.190347217381809e-02  
 4.776643681205300e-02 6.630387109284050e-02]  
 [8.120348879064487e-02 6.956345822462384e-02  
 -2.357481533804585e-03 6.574018195209450e-02  
 -5.048942498603570e-02 4.602056264028722e-02  
 6.004705019158874e-02 1.361654456453548e-01  
 -2.452612278046766e-02 -4.780449513419676e-02  
 -3.749288885598946e-02 5.943337966588186e-02]  
 [-7.130003593100300e-02 8.551483702354165e-02  
 -1.087670650915471e-02 1.405250150729243e-01  
 6.283038863199222e-03 3.133965784849427e-03  
 -2.302527570420544e-03 -2.357503478913817e-03  
 6.072017479265368e-04 -1.088985046632341e-03  
 -1.335518783226083e-03 2.914683873518325e-03]  
 [-6.038020347649314e-02 -9.893076756390586e-02  
 4.529859062964185e-02 -1.445788417788768e-01  
 -2.012127716448736e-03 1.175299694757164e-02  
 1.242453149025945e-02 -1.155581063746455e-02  
 -1.058354887025837e-02 7.346124750836902e-03  
 -1.576395533305513e-02 8.133176915025995e-03]  
 [4.284802911191034e-02 8.560514769285281e-03  
 7.913438478293082e-02 1.746472906683711e-02

-1.106877877421569e-01 6.816830763509120e-02  
1.666727534794383e-01 -6.494568042828688e-03  
4.160476150470879e-02 3.918722065305546e-02  
4.735016043358262e-02 1.503553097204827e-01]  
[-2.825505970975680e-02 -1.019484653898146e-01  
2.754611293931646e-02 -3.209495309484353e-02  
8.594068375919627e-02 4.934013021787433e-02  
4.058588716094277e-02 -1.010840456238964e-01  
-7.916571779444047e-03 3.783545283323828e-02  
-4.126510531722745e-02 1.581901549954529e-01]

9

[4.572675467934201e-02 9.309633989700571e-02  
4.907562678163259e-02 5.117138796346572e-02  
1.431215140397003e-02 -6.903795011199511e-03  
-1.123766959694195e-01 -2.273624192251146e-02  
-8.724814604750386e-02 2.369906404473686e-03  
6.679981965528286e-01 2.161319385103466e-01]  
[-1.350901653438448e-02 -1.076512239311927e-01  
-2.537214956181091e-03 -8.843868199037093e-02  
-2.069490187754018e-01 3.558962299379128e-01  
2.686118706447157e-01 1.473024393102535e-01  
8.167631741395511e-02 1.152967773206514e-02  
-2.394779517196152e-01 8.929890041280542e-02]  
[-2.064897315060681e-03 -1.059006806069787e-01  
9.778627951228130e-04 -6.705388861356479e-02  
1.971992414435620e-01 -4.046734825770887e-01  
-3.737391469122970e-01 -1.463033417974199e-01  
-3.118209372860933e-02 8.681770877273079e-02  
2.748997512856260e-01 -3.976742581400404e-02]  
[-6.381217441385102e-02 -1.920202130508274e-02  
3.796435875094323e-02 -9.481531038731740e-03  
-2.822390238238424e-02 3.805308199998553e-02  
8.727281497901292e-02 -2.503289338947753e-02  
-5.112666393213684e-02 -3.454146306307433e-02  
-9.913254804580918e-02 -1.278847861052115e-01]  
[-7.567336324989030e-02 6.668972415931010e-03  
3.483810849513151e-02 4.614592379110748e-02  
-2.469672273782985e-02 -4.036257533585957e-02  
-7.087403577186059e-02 1.051558232910104e-01  
5.828344905405815e-02 3.350656717788723e-02  
2.635387167219628e-01 -2.037333816549982e-01]  
[8.124304503632815e-02 7.330658959745162e-02  
8.906857229174565e-03 6.902074744831623e-02  
1.126046516551533e-01 3.730079469668415e-03  
-3.109987078582097e-02 5.536272424324788e-02  
-1.110550343964395e-01 5.515337134502914e-02  
-5.763375326739045e-02 1.611477727817574e-02]  
[1.197030259502829e-02 -2.243939158080951e-03  
-6.560935607274014e-01 -9.868173248464779e-02]

-4.124113531117777e-02 4.085777110255066e-02  
 -2.555849075820375e-02 -8.005415246822191e-02  
 2.954837961717583e-02 -7.330604655909576e-02  
 -7.511511279988323e-02 2.686265163270973e-02]  
 [6.989575440549908e-04 1.730811107716215e-02  
 4.670050699104637e-02 2.919632806813372e-02  
 -1.350230784902910e-01 1.033899387376093e-01  
 2.280035795422993e-01 -1.216186583711473e-01  
 4.410709867348273e-02 9.170002039636872e-02  
 8.941091530851261e-01 5.469925102460249e-01]  
 [-5.369150409971314e-02 8.411100707196242e-02  
 -6.430252146232081e-02 1.016975489794365e-01  
 3.453564733398316e-02 -4.449329407190170e-02  
 -3.290366705151150e-02 -2.598821895800395e-03  
 -8.558119874375370e-03 4.681512041804120e-02  
 1.598627962990736e-02 -1.791782787692713e-02]  
 [2.154752905127681e-02 9.530742768752218e-03  
 -4.187208842033856e-02 3.738476528333964e-02  
 -1.189816898415068e-02 2.866132737853138e-01  
 2.118687619386548e-01 -1.006365411224949e-01  
 -1.282667163425142e-01 -2.043212410335986e-01  
 -3.934023602661109e-02 4.613906280917930e-02]  
 [-8.736776030572463e-02 -4.808148406431901e-02  
 -8.080055701757824e-02 -1.651276508753153e-02  
 8.911790511024830e-01 1.781817164837738e-01  
 4.869453622067674e-02 1.748059984872338e-01  
 4.792885688022026e-02 -2.356817413753801e-02  
 1.160867307669000e-02 9.282814431249309e-02]

10

[3.910342224896935e-02 9.307117289201150e-02  
 4.876966867168753e-02 4.949542666910803e-02  
 -3.425592637302049e-02 2.021885253190450e-03  
 -5.081365170633879e-02 1.443687979433681e-02  
 -5.111466207181559e-02 2.434331957855177e-02  
 8.035896772277983e-01 1.287624676614484e-01]  
 [1.331106535590807e-01 -6.848668231707814e-02  
 9.476951837045219e-02 -3.228716491646873e-03  
 -2.756994070036093e-02 1.761367740075048e-02  
 3.589619983826643e-02 1.540167120339633e-02  
 8.152402209073820e-03 -1.167128394466123e-02  
 -7.527625872282723e-03 6.972601175206745e-03]  
 [-2.778535742194218e-02 -1.168675305675063e-02  
 -8.002236890442394e-02 2.011956228664140e-02  
 -6.531646687354997e-02 9.247003012068594e-02  
 8.617992630202670e-02 -5.689762008712791e-02  
 -3.988186551412673e-02 -1.000864630082237e-01  
 5.876840386837359e-02 -1.040404225506524e-01]  
 [1.196408312990668e-02 -2.218552278173725e-03  
 -6.560257020730661e-01 -9.897602544844385e-02]

-4.115251408082491e-02 4.093509823370572e-02  
-2.572103805980026e-02 -8.002794877183689e-02  
2.941162376837778e-02 -7.335865813638733e-02  
-7.506212798295665e-02 2.703960348525964e-02]  
[-9.757884635463153e-02 -4.314845919996978e-02  
-9.735411380117214e-02 -9.290836381301409e-03  
5.335945410321008e-01 1.311181642944623e-01  
-5.871092675654889e-03 1.353623673961151e-01  
6.066693273062696e-02 -5.205295558386811e-02  
1.014582182207726e-01 1.360225575580093e-01]  
[-3.746119656973039e-02 2.399938076327502e-02  
3.581697620534020e-02 3.783987875082562e-02  
-5.124074641387472e-02 1.882832335411813e-02  
-1.035787626717267e-01 -8.525781879953667e-02  
3.209914781932714e-02 1.499009217489631e-01  
1.204339875558187e+00 1.993703213783975e-01]  
[6.405247318557053e-02 5.088160677094664e-02  
-5.956218109406288e-03 6.136941837343325e-02  
1.688224938037079e-01 1.843874484794886e-01  
4.971535922966671e-02 2.080039811031700e-03  
-2.325336904744545e-01 -4.073131639190580e-02  
-9.746573415483104e-02 5.378232768292343e-02]  
[-7.309645741154591e-02 -7.259125425899593e-02  
5.230126667740496e-03 4.000808278428623e-02  
4.285488248380783e-03 7.278836769736021e-03  
4.051295720205238e-02 -2.107938818254041e-02  
1.347718274471708e-02 -1.197659862028658e-02  
-2.993239632708544e-02 6.936783408109247e-02]  
[-4.981830458119554e-02 -2.937581964871139e-02  
8.524625993178023e-04 -4.360938836281971e-02  
-2.025335252200234e-02 -5.151876513530367e-03  
1.269908744268545e-01 1.420125571980280e-01  
6.368413066013617e-02 -7.477781971496383e-02  
2.184455395537680e-02 -8.767923802776097e-02]  
[-5.416033646486459e-02 -7.248871872226181e-02  
-4.052387073636878e-02 -2.436884569723829e-02  
3.505888683149542e-01 1.135219107668803e-02  
3.683321789811714e-02 -8.550814430429508e-02  
-4.112847929627290e-02 1.779213171077414e-01  
-3.553493693219664e-01 2.141927394244118e-01]  
[-2.191615942709003e-02 -1.870839315847350e-01  
-1.734690239391364e-03 -1.973835665391920e-01  
-1.570372817759414e-02 9.435166051469638e-03  
7.755666292782753e-03 3.123739107101083e-03  
1.274604741723906e-03 4.644984418329363e-03  
-7.222306678553900e-03 1.273771882258227e-03]

11

[-1.321559731818602e-03 -1.700829939360597e-02  
4.120551570520271e-02 1.677803652719266e-02

-5.953281737493585e-02 8.272581307173904e-02  
 2.508510750426684e-01 -1.308350076977308e-01  
 3.978774328117422e-02 1.552600454188715e-01  
 3.776595175674088e-01 9.144204563703468e-01]  
 [4.320187133863847e-02 9.003716740535048e-02  
 4.934333850910978e-02 4.922910418038981e-02  
 -2.775780621171582e-02 -6.517764255015875e-03  
 -7.533954561806816e-02 1.307327788231326e-02  
 -7.865748334759536e-02 5.466636182424356e-03  
 7.645448787966301e-01 2.618403785218638e-01]  
 [1.242928448387595e-02 -1.217132869872423e-01  
 4.415763381976270e-02 -8.566653908704319e-02  
 1.278745124188579e-01 3.57328539553371e-02  
 -2.969868720860096e-02 -1.182793901470801e-01  
 2.564676413874645e-02 9.913223365434137e-03  
 7.848065075115540e-02 7.746334621197248e-02]  
 [-5.497131864500943e-02 1.149340780044801e-01  
 -9.714470738887349e-02 7.210754001902384e-02  
 -7.346261111755627e-04 5.406326355587954e-03  
 1.000601366237385e-03 -2.000627619195219e-02  
 -6.525556832611251e-03 1.397244379982767e-03  
 2.874506656476141e-03 -1.149999858472236e-02]  
 [1.681600441972788e-02 -4.481478788271444e-02  
 -2.409753622729320e-01 5.914954028446890e-02  
 1.609642655925991e-03 3.584101265802836e-03  
 2.813646663828486e-03 -2.469711261746750e-03  
 -2.304075658181326e-03 -2.048734284590009e-03  
 2.077198697060932e-03 2.115746235097213e-03]  
 [4.748659769461839e-02 -1.024872909792967e-01  
 1.700127753710146e-02 -5.412705594846879e-02  
 -9.233760293360396e-02 5.011633491589428e-03  
 3.561042952164793e-02 9.689607988315790e-02  
 1.765121072896017e-02 -2.841763664084842e-03  
 -4.508024530381795e-02 -2.506024514635476e-02]  
 [-6.097414019590321e-02 7.086270362296121e-03  
 2.591418573657419e-02 3.851648782891935e-02  
 -3.527746243341408e-02 7.694453169663310e-03  
 -1.255779017462643e-01 1.000945818224987e-01  
 5.840347527939901e-02 4.366335718195004e-02  
 5.930970126112463e-01 -6.536466111415544e-01]  
 [-9.054001347591185e-02 -5.242680302204820e-02  
 -8.686819186216296e-02 -1.888299296694274e-02  
 8.108341010544463e-01 1.344208259890397e-01  
 6.461138144232514e-02 7.561689743721747e-02  
 -1.501490733122615e-02 -5.581977225116517e-02  
 3.940540237892007e-02 7.077567002863466e-02]  
 [7.202212205744271e-02 4.442668684007078e-02  
 1.896875454147326e-03 5.280588911549120e-02  
 1.455828156849177e-01 2.001163020341922e-01  
 3.479612598395258e-02 -4.823919803832752e-03

-2.435313723649886e-01 -5.631689927309059e-02  
 -9.613498526360656e-02 1.464844625169173e-02]  
 [-1.856352775287835e-02 -3.311448837323370e-02  
 5.521568908340821e-02 -7.071728436176698e-02  
 -2.713298932128612e-02 9.975440655816798e-04  
 6.455146636286362e-02 5.456804236129771e-02  
 1.914880308593578e-02 -3.289549891374764e-02  
 -2.417459821758161e-02 -3.316407071991208e-02]  
 [1.194888828992402e-02 -2.265911438607675e-03  
 -6.555918003527352e-01 -9.896226077652418e-02  
 -4.132905117010044e-02 4.111685537725095e-02  
 -2.571893573434410e-02 -8.018823991947037e-02  
 2.950272633770012e-02 -7.362239068869535e-02  
 -7.530817018105976e-02 2.717144572353163e-02]

12

[-9.077719989247231e-02 -5.154092518141244e-02  
 -8.661944682359886e-02 -2.062889625334994e-02  
 8.186582215277409e-01 1.207306923308363e-01  
 7.442593500276136e-02 9.698670224116621e-02  
 6.654540993416860e-04 -6.513448844109078e-02  
 4.699140974197118e-02 9.053318017760700e-02]  
 [-3.340119246897454e-02 -6.382812475974424e-02  
 -6.847218660131682e-03 -1.114206152667451e-01  
 -1.094967164871366e-03 8.316016155516581e-03  
 -3.368881017283125e-03 6.629766608862509e-02  
 6.387797791423013e-02 2.873884656294464e-03  
 2.230967520628874e-02 1.742372460661511e-02]  
 [7.742646384336788e-02 3.601019872846780e-02  
 -4.201982742005204e-03 4.812902961127483e-02  
 1.091870973843288e-01 2.113673799842661e-01  
 9.577685892269251e-02 -6.268489110444814e-02  
 -1.928027065823639e-01 -7.710308355416887e-02  
 -4.768018861509243e-02 -2.487479358582738e-03]  
 [3.821321215946352e-02 8.546191840515811e-02  
 4.930638198725205e-02 4.994858527091024e-02  
 -1.127515138512512e-02 -4.869459925787206e-03  
 -6.412425303405699e-02 -1.640967532321834e-02  
 -9.017130193670729e-02 5.484457352662351e-02  
 1.016280458081401e+00 2.275352918477395e-01]  
 [6.233471088630758e-02 7.869723888729133e-02  
 3.069980483138301e-02 9.424130127606017e-02  
 1.041355250538404e-02 1.588829619980740e-03  
 -2.578208652823908e-02 5.495119019145266e-02  
 -1.645251298101337e-02 -2.184805369035954e-02  
 -7.177869826427161e-02 2.294378184419379e-02]  
 [1.195760758119968e-02 -2.224293155863595e-03  
 -6.560948883237221e-01 -9.888989790086812e-02  
 -4.115498271389314e-02 4.090027572138734e-02  
 -2.569558534377600e-02 -8.004962173081229e-02]



2.942718105901725e-02 -7.330485433630372e-02  
 -7.505744753603741e-02 2.697295611644846e-02]  
 [-5.651487166600156e-03 -1.499610538289746e-02  
 4.504054240314035e-02 1.507682081736673e-02  
 -1.804870937808604e-01 7.075424038719044e-02  
 2.322374805820745e-01 5.257911728701695e-02  
 5.749271444936259e-02 5.287443286667063e-02  
 1.689821262417150e-01 2.132546771652462e-01]  
 [-3.562636241392002e-02 -1.260185610675428e-01  
 3.197717742889877e-02 -1.212381874556833e-01  
 1.421444942175281e-02 4.306511630656369e-02  
 1.127949626728152e-02 -3.607703639071450e-02  
 -9.503483915453003e-04 2.654681119022716e-02  
 -1.405618448613143e-02 3.914986607846505e-02]  
 [-4.491019572332344e-02 -9.026147442462831e-02  
 1.516980504260281e-02 -1.651400046436529e-02  
 7.229298399774722e-02 3.216569185884647e-02  
 1.946922923337892e-02 -6.466354394917090e-02  
 -1.698039002892043e-02 2.107509163210162e-02  
 -9.679784126370733e-02 8.547373739000233e-02]  
 [2.816166408328848e-01 1.457242961211583e-01  
 -8.983319366985127e-04 1.943115402205369e-01  
 3.473263693725796e-04 -6.613111458165076e-04  
 -1.314935578206474e-03 1.022047527844044e-04  
 1.823590984014079e-04 3.773620037392467e-04  
 -9.277799961289997e-05 -1.700076417198115e-04]  
 [-6.030921530454795e-02 2.880067808735838e-02  
 3.078166875740053e-02 4.503519007716389e-02  
 1.069728009633998e-02 -1.306852677221891e-02  
 -1.150036024303811e-01 -2.738577769800902e-02  
 9.818900617510260e-03 7.095377159955546e-02  
 6.683406373863088e-01 -7.556516447542050e-02]

13

[-9.214681940101786e-02 -4.922722547189493e-02  
 -8.945990822217137e-02 -1.563950763308994e-02  
 7.449791223250029e-01 1.648075842504744e-01  
 6.918288211003516e-02 9.941479072173610e-02  
 4.252869830270773e-03 -6.808364260906968e-02  
 5.460159216646698e-02 7.868012223238759e-02]  
 [1.268151841865236e-02 1.327715574340496e-01  
 -9.325291452860265e-02 1.478029531970605e-01  
 -2.379683173459574e-03 -1.005948032989687e-02  
 1.164518232378447e-02 9.476848992598019e-03  
 9.781888140913977e-04 3.895034829871604e-03  
 6.078031896476502e-03 5.602793293061072e-03]  
 [1.402048494374713e-01 6.793181832513054e-02  
 -9.442535155445454e-02 -4.662108012504770e-02  
 -9.844389881940787e-04 -9.897158217043478e-06  
 6.073064875059532e-04 2.093223088494240e-03

9.547039684253089e-04 -1.332195269815665e-04  
-6.528482445980754e-04 8.096554633197092e-04]  
[3.721040648019038e-02 8.935943623419239e-02  
4.916101751227073e-02 4.877760861793232e-02  
-3.771223132690911e-02 1.347150296654787e-02  
-2.537949452280741e-02 2.438097372114471e-02  
-7.255031179718696e-02 3.967174723933424e-02  
9.193730640068388e-01 1.820071715847142e-01]  
[1.398568548695791e-01 -2.291599033909708e-01  
2.353348617176300e-01 -1.813951169553108e-01  
2.175079689572865e-03 -2.329341879673062e-03  
-2.588588380760071e-03 1.480762371121164e-03  
-5.139857240177349e-04 -5.954340178696540e-04  
1.730765387426174e-04 -1.028992844417774e-03]  
[-3.848006883425686e-02 -1.001897716137505e-01  
1.021861759646191e-02 -2.242548555855974e-02  
8.000557696137152e-02 3.939840392171421e-02  
4.417833647060165e-02 -1.145779837220513e-01  
3.727929718414640e-03 5.228212656719636e-03  
-1.295558107188730e-02 1.427813334645528e-01]  
[1.197252981894160e-02 -2.233038480333436e-03  
-6.561308349798202e-01 -9.902108438128585e-02  
-4.110079090709432e-02 4.091660778575590e-02  
-2.570401525111427e-02 -8.000003858913968e-02  
2.936228634983307e-02 -7.331359885946483e-02  
-7.499539442793392e-02 2.702881743715805e-02]  
[-2.725692009123955e-02 -3.915829211398272e-02  
3.089797623085001e-02 -9.793096584314875e-02  
-2.724976713473427e-03 1.712286880229055e-02  
4.087678475581275e-02 3.453153232828615e-02  
1.788830516087924e-02 -2.706184917286191e-02  
-5.303844575851591e-03 -7.012507859995603e-03]  
[-5.241202641847691e-02 3.005985932783780e-02  
3.262060086848494e-02 4.319393394836232e-02  
-4.767238061036321e-02 1.819311738141672e-02  
-6.773918612083149e-02 2.644365401928367e-03  
2.250665314710642e-02 9.088144671914689e-02  
8.581755273438377e-01 3.079543408288487e-02]  
[2.678983609673982e-03 -6.947979686360330e-02  
1.695018507462343e-02 -4.080436580717792e-02  
-5.896770148126017e-02 -3.806331671388585e-02  
8.043656262632401e-02 1.056527655701666e-01  
9.769775508491015e-02 1.163426853420143e-01  
-5.225935964341576e-02 1.804682034499423e-01]  
[6.527926468674106e-02 3.372065632484823e-02  
-7.826218191079043e-03 4.306583550705980e-02  
1.661811404827230e-01 2.668408954942382e-01  
7.238388557769525e-02 -1.014509055196123e-01  
-2.601970672354132e-01 -9.467593514754981e-02  
-7.479309549584379e-02 4.932533446986949e-03]

14

[-5.208380073057799e-02 2.985180857725829e-02  
 3.231507827844550e-02 4.049281332406648e-02  
 -5.964927132941356e-02 1.085920781523590e-02  
 -9.786281810628648e-02 -1.561847287601779e-02  
 2.102818478919676e-02 9.971856549916540e-02  
 8.824395030099766e-01 4.897306266440980e-02]  
 [-1.058265106374768e-02 -4.840690803599735e-02  
 1.509537285340578e-02 -5.096397384466844e-02  
 -3.265120048895439e-02 -1.315202591070684e-02  
 1.060919263017253e-01 2.055013131366624e-01  
 1.537282176484484e-01 4.403613952843486e-02  
 2.275765928525256e-02 8.875102133121277e-02]  
 [-1.676540920089749e-01 -3.674044504897662e-02  
 1.175588643606532e-01 -3.954048855862902e-03  
 3.314286983666598e-04 -1.461450257253283e-03  
 -1.392484530237366e-03 -3.847172950548993e-04  
 -8.271059445971069e-04 7.611652538731621e-04  
 1.159547344218537e-03 5.885563176399430e-04]  
 [-9.366454542477505e-02 -5.261122504918875e-02  
 -9.130875669068940e-02 -2.099633058784419e-02  
 7.460645303536062e-01 8.878194301293103e-02  
 5.498097107290755e-02 7.343132924736689e-02  
 7.450169367549558e-04 -6.246152490085260e-02  
 5.962033259258234e-02 9.260963576249853e-02]  
 [1.193254557547401e-02 -2.220108188562863e-03  
 -6.559035822240095e-01 -9.898051993534467e-02  
 -4.118136709745137e-02 4.100088096933515e-02  
 -2.580004592115757e-02 -8.009914527126023e-02  
 2.946861993118782e-02 -7.341178173447847e-02  
 -7.514348335550783e-02 2.708681220314051e-02]  
 [-3.730998897199271e-02 -9.027252022391365e-02  
 1.945931609954636e-02 -3.970691796880479e-02  
 1.125146260103010e-01 1.069347545320087e-01  
 9.484286214667875e-02 -1.590889745368784e-01  
 -4.073040709140627e-02 5.157640147511078e-02  
 -1.312756022792071e-01 2.124126695555162e-01]  
 [6.844218706936954e-02 2.565249785133538e-02  
 9.825344455414598e-04 4.152429764680500e-02  
 1.077454491654253e-01 2.912058331869154e-01  
 8.484080510920114e-02 -1.200926770517255e-01  
 -2.169314825841325e-01 -1.300963040394004e-01  
 -5.161331665595380e-02 -2.790986615392572e-02]  
 [-1.780684531131935e-02 -1.779344997373292e-02  
 -2.168647093879474e-01 -1.450488676855761e-01  
 -3.737812931190602e-04 -6.549302078667968e-04  
 -7.911552369734169e-04 -1.734576401194683e-03  
 -4.366150154795631e-04 2.480353097806073e-03  
 -1.418645147410753e-03 -4.914112136258232e-04]

[5.404540537178195e-02 9.247650823608460e-02  
 -2.646310751506837e-02 7.454331059537483e-02  
 1.363960752151906e-02 -1.230983753298116e-02  
 4.134310292955302e-02 3.289191556934916e-02  
 -2.107949817764301e-02 1.670848796830502e-02  
 4.373210722177106e-03 3.774249028056072e-02]  
 [3.673145208016824e-02 8.909971768443495e-02  
 4.847849153816097e-02 4.870659816083890e-02  
 -3.210240726749811e-02 9.513418701564892e-03  
 -6.390053148639499e-02 2.991298387456044e-02  
 -7.380225763266746e-02 3.786236988993855e-02  
 9.195046793129734e-01 1.636229713079083e-01]  
 [9.330869591182076e-02 -7.644809222571290e-02  
 1.632465081252725e-01 -2.887431097182377e-02  
 -1.253889801486550e-02 -1.042884978841791e-02  
 5.547023797230155e-03 1.892735596886470e-02  
 -7.055345542349051e-03 4.981575415386778e-03  
 -1.296271633626892e-02 1.678621695259233e-03]

15

[6.688958036454698e-02 3.794980460254990e-02  
 -4.894422222342605e-03 4.665198922926009e-02  
 1.443186414442352e-01 2.720424772803148e-01  
 1.240945044347678e-01 -1.576139677254877e-02  
 -2.350815736075557e-01 -5.367627363681082e-02  
 -8.163776618857679e-02 8.271897492307968e-02]  
 [-6.060139356824657e-02 3.185904040690073e-02  
 3.168618418644693e-02 4.370056505025275e-02  
 -5.500625953253190e-02 -1.359526117270917e-02  
 -7.371782173493578e-02 1.574185772419426e-02  
 6.608571438832112e-03 8.012477897242459e-02  
 6.836033836045105e-01 2.375156359767311e-02]  
 [1.194312251493723e-02 -2.229367771828645e-03  
 -6.560141180458845e-01 -9.897853108587913e-02  
 -4.115125765404744e-02 4.096217377064545e-02  
 -2.573490125330032e-02 -8.007016423063486e-02  
 2.940625461155138e-02 -7.335819352493316e-02  
 -7.507803834377447e-02 2.704208433257011e-02]  
 [1.055293198417489e-01 -3.744811393019930e-03  
 1.064133594137637e-01 4.758731698591961e-02  
 -1.353640647687385e-02 5.389031229469708e-02  
 4.930897798315591e-02 -4.888391176385919e-02  
 2.481377965272230e-02 1.286584582708144e-02  
 4.788325747048727e-02 2.121110173839158e-02]  
 [3.680675872869117e-02 8.681686685674313e-02  
 4.894941849802912e-02 4.876885230043317e-02  
 -7.441511746928668e-02 -5.818641562612857e-03  
 -3.648497779434702e-02 6.036517437139170e-02  
 -9.100062208456004e-02 5.903842281168675e-02  
 9.692088516016442e-01 2.515739644757121e-01]

[5.306201665145398e-04 -3.425925513743167e-02  
 -4.868368984858525e-02 -3.387694868516364e-02  
 -5.982578363546236e-02 -5.555875741462219e-02  
 -6.544194420726112e-03 -3.176832695824203e-02  
 -5.894326355952534e-02 2.455725555180630e-04  
 -6.387290082952780e-02 -9.208573131980677e-02]  
 [-2.390104431424012e-02 -1.673883188255979e-01  
 1.300782149489653e-02 -7.566873051134158e-02  
 3.079798928823396e-02 -5.418683201740709e-02  
 -3.221476533810183e-02 -1.109351878648951e-02  
 5.356126886754700e-03 -1.247487330089937e-02  
 3.832202825273179e-02 1.539913037864297e-03]  
 [-3.361985184295029e-02 -5.621795865749387e-02  
 6.435951922544144e-03 -7.369771298865478e-02  
 -5.645288585452129e-02 9.928417921315673e-03  
 1.134022775124578e-01 1.370384638944334e-01  
 4.345168513122152e-02 -6.321132580217403e-02  
 -2.003116549441684e-02 -7.126229717299747e-02]  
 [1.313178338771559e-02 -9.748070593419282e-02  
 2.319116191215050e-02 -5.175290876461757e-02  
 1.748839719604438e-01 1.433692941728214e-01  
 2.914707191037724e-02 -1.165492268972841e-01  
 1.186596694339601e-01 1.052907837266733e-01  
 7.465514191341476e-02 2.979810658794505e-01]  
 [-9.582549995928082e-02 -4.994569390540986e-02  
 -9.158305776521462e-02 -2.136381319268587e-02  
 7.523636036784301e-01 1.192646449828635e-01  
 5.650398056696341e-02 7.446049189655966e-02  
 8.211348387678627e-04 -6.268647589874157e-02  
 4.443313680875698e-02 1.025730340584967e-01]  
 [4.066898423628100e-01 -2.392171094809463e-01  
 1.249651128503876e-01 1.829326879663159e-01  
 -1.777794907034241e-04 -8.883734541846399e-06  
 1.395042099347328e-04 1.668918871515133e-04  
 1.556457514423879e-05 -2.814276536031529e-06  
 -4.476030241771088e-05 2.089020016033904e-05]

16

[-3.851964413824902e-02 2.536151123214074e-02  
 3.678230782068901e-02 3.867899151211022e-02  
 -5.563469782288250e-02 2.380560216417209e-02  
 -9.340962343407379e-02 -1.009931992465492e-01  
 1.006828782346003e-02 1.415352239637264e-01  
 1.130123725268680e+00 2.214016686002282e-01]  
 [-1.198591552517166e-01 -2.236178690645383e-03  
 -3.033422804797025e-02 -2.092449781942624e-01  
 -8.003714623681759e-04 -1.243786804906760e-04  
 1.116252040646794e-03 4.246261326782737e-03  
 2.638109788749515e-03 -8.004475209608839e-04  
 2.933646242321622e-04 -2.659290273142544e-04]

[-9.016514502300807e-02 -5.990716918534430e-02  
-8.536694832966406e-02 -2.344944607616695e-02  
7.757746263735146e-01 3.048143582797986e-02  
1.199341393261260e-01 7.734380045605958e-02  
-9.243365655473805e-03 -9.402410607831704e-02  
9.138330117873640e-02 4.807553679715960e-02]  
[4.230605864930236e-02 -2.383535325936717e-01  
1.057957522757436e-01 -1.410115267409779e-01  
1.036814363161958e-02 -3.860345897831840e-03  
-6.991809136842140e-03 -7.394574951596902e-03  
-1.750778673365243e-03 8.784532441873992e-04  
2.659832235391359e-03 8.133292496608229e-04]  
[-1.574703143904024e-02 -7.317394304372579e-02  
-3.767043777935022e-04 -4.730874784702838e-02  
1.546294174848829e-02 9.156182357465358e-02  
3.326281260210590e-02 2.062530747923885e-01  
1.593965208239776e-01 8.639306098768360e-02  
2.226621424809136e-03 1.697535703484639e-01]  
[-6.461535182225237e-02 -5.523835581907027e-02  
3.419836387815134e-03 5.175020531075381e-03  
-3.822640857970967e-03 3.742711206690447e-02  
1.574482749080529e-01 -6.595799173095245e-02  
-3.883750680197319e-02 -8.661418091766784e-03  
-2.904257450261964e-01 3.248358620726698e-02]  
[-9.426239954948509e-02 -1.765329304114634e-01  
-2.183897485505668e-01 -4.074130274911202e-01  
-4.882628171310843e-05 -3.842831180544874e-04  
7.214161377831675e-05 4.746518169483009e-05  
-3.578042218698609e-04 5.134326961871129e-05  
6.561081252364879e-05 -1.991038877437649e-04]  
[3.842555230140467e-02 9.191467088986161e-02  
4.858956355313073e-02 4.883068921512079e-02  
-3.042354784731134e-02 8.841044003991192e-03  
-5.444102052115476e-02 1.062336501763140e-02  
-5.622597411666844e-02 3.396751147455721e-02  
8.392080426204814e-01 1.354223616740637e-01]  
[6.263614793402203e-02 3.985704761378104e-02  
-8.901446293301236e-03 5.363187186276806e-02  
1.722380800212669e-01 2.806212491546570e-01  
4.310485949153881e-02 -5.286128666447538e-02  
-2.609017808471100e-01 -9.164570185525507e-02  
-9.752096290648185e-02 1.600649578470584e-02]  
[1.200481164871335e-02 -2.198332311137677e-03  
-6.561332797449685e-01 -9.883401871727073e-02  
-4.114399668238827e-02 4.085383319644195e-02  
-2.565199348025424e-02 -8.004906868832970e-02  
2.939281787974877e-02 -7.328054807398754e-02  
-7.502712666632415e-02 2.693454106577095e-02]  
[-2.907373278422141e-02 1.088830929036525e-01  
-8.635677012017276e-02 1.100205195103004e-01

-4.017099456233853e-02 1.065852228341720e-03  
 2.345562266632218e-02 -7.611511127981249e-03  
 9.928801317837483e-03 -2.257923866196908e-03  
 1.445450492698031e-02 -5.361493061667761e-03]

17

[-6.671650900960712e-01 -9.871207057820791e-01  
 -4.623811488697715e-01 -6.879907970766871e-01  
 1.588072166895143e-05 1.849578077310373e-06  
 -1.195278989547564e-05 -1.425246517738627e-05  
 3.380386074182274e-06 -1.282167672072918e-06  
 -2.566012970917913e-07 1.373609499114522e-06]  
 [-8.305838505413944e-02 8.023574389789253e-03  
 2.055316532975766e-02 4.302970278862609e-02  
 -3.747548410765468e-02 -5.679403514665331e-03  
 -1.941018732370823e-02 8.631006090892392e-02  
 2.866366448994461e-02 2.065648057759587e-02  
 2.244046442637381e-01 -2.797243958502147e-01]  
 [4.494183710286057e-02 8.611971104079659e-02  
 4.947127820247893e-02 4.725903817242958e-02  
 -2.120862790108594e-02 -2.049181817565243e-02  
 -1.117030974751909e-01 3.144316659763553e-02  
 -8.843714143122858e-02 -7.121456819463145e-04  
 7.505301779253107e-01 3.491702192675676e-01]  
 [-1.543311039287431e-03 1.428293229734257e-02  
 5.499545165220226e-02 3.594599364809389e-02  
 -3.910895652346424e-02 1.154003878013346e-01  
 7.841403061973234e-02 -2.109559427605501e-01  
 2.644007359403850e-03 6.817724024785817e-02  
 5.565379453521600e-01 2.416072686236480e-01]  
 [-9.353809739597749e-02 -5.261930939794359e-02  
 -8.671161655389455e-02 -2.062567851006271e-02  
 8.307089560440333e-01 1.435367429771806e-01  
 4.830538228096830e-02 7.438946255308848e-02  
 3.297138252044030e-03 -6.058124715435997e-02  
 1.314974993388383e-02 1.074675287050656e-01]  
 [7.098268700729458e-02 3.039923296460931e-02  
 3.247568643273049e-03 4.493360795617717e-02  
 1.383883003639482e-01 2.982668980024631e-01  
 1.093285220630125e-01 -1.846087781467863e-02  
 -2.793649304552135e-01 -1.201789868548273e-01  
 -1.002368994498955e-01 3.600709419322174e-02]  
 [9.727095800634706e-03 -1.503866732314349e-02  
 1.656870053860277e-02 1.667141342048630e-02  
 -2.692576623812703e-02 -1.297278098327072e-01  
 9.789119412000155e-02 1.006559939935260e-01  
 1.130395357890607e-01 1.199196620003278e-01  
 2.959787749606956e-01 1.134229116330311e-01]  
 [-2.618549890118292e-02 -4.886559732206221e-02  
 -2.328940837593011e-02 -1.191827593912993e-01

-2.161296093545449e-02 -2.767173385232885e-03  
 -1.587116013181890e-02 4.148193506470361e-02  
 3.277206433817340e-02 1.516681982269698e-02  
 -9.015356737222072e-03 1.051388146592955e-02]  
 [-4.745821796988343e-02 -1.426815677284813e-01  
 4.906180866144049e-03 -1.091364166428351e-01  
 2.048922058296073e-02 7.125856660093344e-02  
 3.699085916346627e-02 -4.235651346104969e-02  
 2.076697867724984e-03 2.318529764917673e-02  
 -3.850205083596358e-02 3.964427968866693e-02]  
 [1.196898594271879e-02 -2.234393792928032e-03  
 -6.560758818195326e-01 -9.878444767276189e-02  
 -4.118295288905117e-02 4.087480336978008e-02  
 -2.565315976405617e-02 -8.007648280447438e-02  
 2.947533945929061e-02 -7.329211012622967e-02  
 -7.509385121908041e-02 2.692021576628381e-02]  
 [3.125198754123169e-01 2.836639273621228e-01  
 8.313175676414880e-02 1.919626635480578e-01  
 -2.888928598571813e-04 -3.840989007462305e-04  
 -3.807746862651976e-04 1.229784552724792e-03  
 -6.242873796134388e-05 -1.842808593311345e-04  
 -3.117090994970465e-04 3.418664789546871e-05]

18

[8.514411145392095e-02 5.483966133669910e-02  
 6.357599144184295e-03 6.404819643842655e-02  
 5.194842668923227e-02 1.440708049105704e-01  
 4.076962841018052e-02 6.476798105449244e-02  
 -1.348579804335861e-01 -7.595271331161826e-02  
 -9.379564231924861e-02 1.495062226858738e-02]  
 [-4.468310537997865e-02 -6.814048716283695e-02  
 -5.712423948346055e-03 -4.762895625778293e-02  
 1.848297677980646e-01 2.149264688940136e-01  
 4.423097915777992e-02 4.286101852437778e-02  
 1.036003991574824e-01 1.833101425630662e-01  
 -3.229080479815677e-01 3.998651380871290e-01]  
 [-8.327341746939446e-02 -5.502763818523958e-03  
 4.041030989328516e-02 5.013055501261948e-02  
 -2.144679410590770e-02 -5.361925964650754e-03  
 -8.476174415188692e-03 5.086641929428701e-02  
 2.305694090404860e-02 3.529776752293809e-03  
 3.934130702203746e-02 -1.248562879841719e-01]  
 [1.308251819553793e-01 -5.340523887952714e-02  
 5.660244680980354e-02 1.304042580542519e-02  
 -2.199542998370435e-02 4.502213705062331e-02  
 5.495885921914819e-02 1.608306325288427e-02  
 -7.905265868338575e-03 -2.872330703087238e-02  
 -1.788100218052084e-02 8.534303377658611e-03]  
 [-6.654802111202178e-02 -5.291449099328489e-02  
 9.783344737557536e-04 -5.621062212250741e-02



-7.573155706965835e-02 -2.065130492931295e-02  
 1.283323459869420e-01 6.184120382602262e-02  
 -1.384733567399067e-02 -1.096674351440909e-01  
 8.319546240993919e-02 -1.688704205255601e-01]  
 [-9.492158755453375e-02 -5.527967249335046e-02  
 -9.258034732743027e-02 -2.447362117456324e-02  
 7.286498474995055e-01 1.627433958612261e-02  
 6.687996842115870e-02 5.486663452259279e-02  
 -3.357159395983501e-03 -7.490764885394655e-02  
 7.197174529655542e-02 1.008035379801801e-01]  
 [4.145802710540346e-02 9.391975366736380e-02  
 4.918012076150913e-02 5.065065445824681e-02  
 -1.199696093552252e-02 -9.831556280218128e-03  
 -8.304005529629914e-02 7.745838798250027e-03  
 -6.262743837477004e-02 2.349123543517360e-02  
 7.362284026703129e-01 1.362777352178767e-01]  
 [1.435128633909160e-01 -5.925162715934126e-02  
 2.245064081235378e-01 -5.419890883856054e-02  
 -2.361734428328972e-03 -4.231517256955354e-03  
 1.319103811400301e-04 3.569085204729753e-03  
 -1.898987597846745e-03 5.307622058840035e-04  
 -2.851867406596798e-03 4.306731608954768e-05]  
 [1.370522611217380e-02 -1.035520568310632e-02  
 -5.759197920407284e-02 -5.761690113180536e-03  
 6.293833300941719e-02 2.059473237673758e-02  
 -2.279479736056719e-02 -7.131445107918191e-02  
 -7.229324227948795e-02 2.190162536460597e-02  
 3.339145116214801e-02 -2.494557252444746e-02]  
 [-2.575775803834583e-02 2.494187059510129e-02  
 3.299852775849910e-02 3.860590421107797e-02  
 -5.179201956004547e-02 6.855275049552949e-02  
 2.546914019742445e-03 -1.675038244460389e-01  
 -1.529172998623016e-02 1.220309425364215e-01  
 1.165939359503580e+00 2.763146191050316e-01]  
 [1.195462341905946e-02 -2.236041393939003e-03  
 -6.559173276522191e-01 -9.874234391074530e-02  
 -4.124316265513601e-02 4.092401563830494e-02  
 -2.563992244779089e-02 -8.013663458774388e-02  
 2.952912686601588e-02 -7.338793306362790e-02  
 -7.518999968380757e-02 2.694782143222021e-02]

19

[1.014835776770097e-01 8.021935331809441e-02  
 7.021065773087165e-02 1.138516964792511e-01  
 2.837053113101342e-02 2.595115443959316e-03  
 -4.105892887748580e-02 -6.523550341035517e-03  
 -8.703449488620283e-03 -1.536141043194832e-02  
 -1.406482975731775e-02 -1.374079002836094e-02]  
 [-3.779615331805611e-04 -7.360530226850895e-02  
 6.993981994778692e-03 -4.980986506127624e-02]

-5.886193204047552e-02 -1.238401089930615e-01  
-1.112807413146007e-01 1.773313841403164e-01  
1.470391729353904e-01 8.107019088941853e-02  
1.320686416207924e-01 3.594588331638201e-02]  
[-4.351893983429656e-02 4.391367748623658e-02  
3.747854565008075e-02 4.498156461688545e-02  
-7.991359746170072e-02 -1.145520355211542e-03  
-2.905723835621488e-02 -1.529397954561003e-02  
-2.308701029886960e-02 1.165465054394664e-01  
8.086642512014129e-01 3.507459492021399e-01]  
[-4.275879130134045e-02 -8.966754441990750e-02  
2.605500785031312e-03 -6.859890657555816e-02  
7.467533515879668e-02 2.320116185287827e-01  
2.202293583236600e-01 -6.144056137537862e-02  
-1.736472937895642e-02 -3.032675491699549e-02  
-1.638093359359012e-01 8.401162419854277e-02]  
[-6.084837573176493e-04 -1.222143048506628e-02  
-7.745981877263518e-02 -1.546332373385177e-01  
-2.092132064517976e-03 2.938677078732694e-03  
-6.580602635908900e-03 -9.139171153569510e-04  
1.228127552853402e-03 5.905618440766004e-03  
-6.604564645448277e-03 3.659306746986715e-03]  
[9.614471157335132e-02 1.200128427953045e-01  
-5.923900352282822e-02 -1.660734781957121e-02  
-5.229876687380509e-04 2.009180384550261e-03  
5.765759433961446e-03 -4.021418689693103e-04  
5.846509529026942e-04 -2.176278024817821e-03  
2.590946216991797e-03 1.104813998997065e-03]  
[6.554717216592768e-02 3.361895151258557e-02  
-9.352803915608120e-03 4.645051829552536e-02  
1.534916378544833e-01 2.639270799902138e-01  
9.360368609766737e-02 -9.776939915006815e-02  
-2.368580615443214e-01 -9.040119710572242e-02  
-5.468678624516916e-02 3.033290213106288e-02]  
[1.194613881677293e-02 -2.242320012083421e-03  
-6.558476715147182e-01 -9.882128353693487e-02  
-4.125081089042028e-02 4.097477362822612e-02  
-2.571303764628880e-02 -8.019798238288670e-02  
2.948641128741268e-02 -7.339868118395548e-02  
-7.521327319070577e-02 2.699671428062517e-02]  
[3.344191970381558e-02 9.199258402399863e-02  
4.943732125166712e-02 4.834886368727623e-02  
-5.077785301081431e-02 3.681486832389785e-02  
6.635613051192743e-03 1.329674372680386e-02  
-3.492225903772441e-02 6.427153914559255e-02  
9.644461030044728e-01 4.561382607986297e-02]  
[-9.449514649219838e-02 -5.443059290495521e-02  
-8.968185174755437e-02 -2.581745738145666e-02  
7.908441319722837e-01 4.237076056028930e-02  
7.338467778433262e-02 4.868441627859561e-02

-1.243769359482448e-02 -6.915992629125982e-02  
 5.143936825429999e-02 9.794682807790130e-02]  
 [-1.094050454086055e-01 -8.063254305181221e-02  
 4.818995356952097e-03 2.189501208992138e-02  
 -1.216360672199371e-02 1.163249993038612e-02  
 1.197111021593090e-02 6.875321998261461e-03  
 -8.578320679296132e-04 5.185841492744917e-03  
 -2.738935203059591e-02 -1.755249425354558e-02]

20

[-6.128038852898820e-02 2.191295634627189e-02  
 2.610043429052034e-02 4.220481878180030e-02  
 -4.535408842478427e-02 -1.053746798624794e-02  
 -8.870155102826850e-02 4.800772408800671e-02  
 3.519584236037013e-02 7.599224694001498e-02  
 7.292699917317032e-01 -2.234501944857122e-01]  
 [1.197739479672388e-02 -2.213652941048827e-03  
 -6.562197392719080e-01 -9.892892093959337e-02  
 -4.110172714129723e-02 4.087169973143606e-02  
 -2.569421945133152e-02 -7.998940746049928e-02  
 2.938227427890008e-02 -7.324592543635275e-02  
 -7.497468332288837e-02 2.696021755929710e-02]  
 [-6.752132248644428e-02 -1.595294964269741e-01  
 -4.561825537471415e-02 -1.641808067387195e-01  
 -2.048258097403836e-02 1.602501380393939e-03  
 5.256726224166297e-03 4.386515364174601e-03  
 -5.982387409264283e-03 6.178068328633768e-03  
 -7.973869961660926e-03 -6.366076088177965e-03]  
 [6.676833470559393e-02 3.060950355998777e-02  
 -2.254782194708602e-03 4.625882239341907e-02  
 1.200005342779117e-01 2.700596513881693e-01  
 -6.957601069870087e-03 4.221016423246535e-02  
 -2.640958490430653e-01 -1.259226277944693e-01  
 -1.691308025780800e-01 -3.424630851014134e-02]  
 [3.696119831713739e-02 1.098654850145664e-02  
 8.266075808588060e-02 4.117507683017296e-02  
 -3.808536493068792e-02 6.076910431694089e-02  
 7.772980336258284e-02 -6.941399777106648e-02  
 2.969682517071118e-03 1.776934287093036e-02  
 1.186315310068357e-01 8.951731593172223e-02]  
 [4.007238871307589e-02 8.874370392906575e-02  
 4.834559600611082e-02 4.913332865118591e-02  
 -2.698290087761030e-02 -2.257876249675371e-02  
 -8.437813972136882e-02 4.022334476261769e-02  
 -8.293299729237327e-02 3.095982662408654e-02  
 8.409577658507864e-01 2.505706511576906e-01]  
 [-4.092051602371947e-02 -3.434432887537749e-02  
 -2.364718883517737e-02 -1.248401076709733e-01  
 -1.200841470758067e-02 -8.847754303242895e-03  
 -9.813418856379789e-03 3.964649479329482e-02]

2.404377628330423e-02 8.194084150703884e-03  
 -1.400574838390997e-03 -8.436414850157096e-03]  
 [1.995856993839091e-02 -4.812532906087037e-02  
 1.040844464013267e-02 -2.425609987363500e-03  
 -2.765526974156750e-02 1.535304628203396e-01  
 4.600192783789414e-01 2.286178014757903e-01  
 4.228960749853852e-02 1.027436156089788e-01  
 -3.072814225367014e-01 4.681750455185320e-01]  
 [-1.718959378290336e-02 5.648281329186051e-02  
 -5.738544165016415e-02 5.029317802841745e-02  
 -2.981592696908699e-02 -2.037180260595002e-02  
 -1.291772347870477e-02 -8.449954616305937e-02  
 1.873798373359325e-02 1.418825360559956e-02  
 5.096733051335958e-02 -8.380653271612173e-02]  
 [-4.510189578813285e-04 -8.876539236472184e-02  
 1.760136967134465e-02 -2.090823208988091e-02  
 1.632098102858166e-01 -1.373994811340967e-01  
 -1.802050324377506e-01 -2.881126035893092e-01  
 5.346627348366061e-02 -7.182025069351663e-03  
 3.766888189273045e-01 1.276039785704400e-01]  
 [-8.978813962240963e-02 -4.911332463349664e-02  
 -8.646425796619840e-02 -1.524687798024925e-02  
 7.600746454608410e-01 1.831907934097761e-01  
 6.356153415422963e-02 1.025698446322570e-01  
 -8.966879093422168e-03 -5.751941237548498e-02  
 6.168708370056419e-02 3.854288166322247e-02]

21

[-5.799928632946030e-02 2.677177250034089e-02  
 3.194251895311757e-02 4.518062918386929e-02  
 -4.906668758919022e-03 8.010229785006923e-03  
 -7.072902912893893e-02 -1.450993451726150e-02  
 2.303249537335811e-03 6.684389364321018e-02  
 7.147919237629291e-01 -1.209039370636937e-01]  
 [-7.546280656729137e-02 -5.621356909717167e-02  
 -6.476200427604739e-02 -2.952282668838268e-02  
 9.360540148252775e-01 6.373342153073673e-01  
 7.170300626379400e-02 2.040068213391378e-01  
 1.657949055060478e-02 -6.765657089827503e-03  
 -1.401270341077894e-01 9.984140891848167e-02]  
 [-4.099158576814926e-02 -1.087341918704643e-01  
 1.443893694563629e-02 -3.813277698525742e-02  
 9.333492705451757e-02 6.252845154089821e-02  
 2.459139302077317e-02 -1.152397807212374e-01  
 -1.912225072842650e-02 1.853038356743255e-02  
 -3.334998058419466e-02 1.084845577944927e-01]  
 [-9.228221600337769e-02 -7.924542335199920e-02  
 -9.129608385453487e-02 -5.871148421578037e-02  
 -2.946185416149819e-02 -4.447053223518150e-01  
 -7.286166378224996e-03 -4.060608183893909e-02

-4.604024663887305e-02 -2.082588982676020e-02  
 9.767650081675029e-02 -5.782060769454711e-02]  
 [1.747823042723426e-02 -6.583910072320373e-02  
 5.580079818968588e-02 -1.658026100572013e-01  
 -2.246160145026381e-03 6.376380027919798e-03  
 9.309795202735600e-03 1.268043780003003e-02  
 7.847278525348269e-03 -8.717522180515499e-03  
 2.287015899258700e-04 -2.081606837202630e-03]  
 [3.864240240926159e-02 8.788432736716151e-02  
 4.896148292625809e-02 4.895719656362024e-02  
 -1.958090566118241e-02 1.456817085990381e-02  
 -3.866289048946833e-02 1.977378687818325e-02  
 -9.921416678893345e-02 2.519112574891623e-02  
 9.087433125019214e-01 2.364854961197815e-01]  
 [2.293044962039258e-01 4.259189204352454e-03  
 3.062577497388350e-01 1.698299938607510e-01  
 -1.127317197627284e-04 7.854989881673858e-04  
 4.074202335006073e-04 -2.192588790191961e-03  
 1.779329231229563e-05 6.138295666176290e-04  
 6.821106587505279e-04 1.597375878549533e-04]  
 [-9.353159836646145e-03 -2.311762254381098e-02  
 1.803482557315643e-02 2.923951264510298e-03  
 -3.216608491523756e-01 -3.675811261274418e-02  
 1.704581815805619e-01 9.286177870960161e-02  
 2.129079757339489e-01 4.289959020516583e-02  
 2.197418117072610e-01 3.417778737735952e-01]  
 [2.946399998681754e-02 1.760876107634238e-01  
 -1.378097941175528e-01 1.001157780346414e-01  
 -3.075947034193468e-03 4.313456626956672e-04  
 6.841729392305360e-03 1.800988941675231e-03  
 9.286236149572297e-04 -1.536083991295169e-03  
 2.328837571246989e-03 8.716920593314465e-04]  
 [6.796581106246409e-02 4.000237535263610e-02  
 -5.730127059173968e-03 4.417762364749606e-02  
 1.946063134519022e-01 2.208414334789645e-01  
 5.696394513093533e-02 -9.485393793337017e-02  
 -2.615385484549637e-01 -5.080572078520014e-02  
 -7.821730497108127e-02 1.130635781239722e-02]  
 [1.193795351785700e-02 -2.215677322709813e-03  
 -6.561374360998300e-01 -9.884424848633464e-02  
 -4.115142244082306e-02 4.087665383440044e-02  
 -2.569772875172775e-02 -8.007515550295577e-02  
 2.943812867400239e-02 -7.327250140445475e-02  
 -7.505771045288791e-02 2.694359128010276e-02]

22

[-4.128769247128421e-02 -5.866528649086302e-02  
 -5.803287410060640e-02 -1.594839517333116e-01  
 -6.852566912759926e-03 -9.251680985615580e-03  
 -2.375194291517185e-02 5.775901401723091e-03]

6.231283617529160e-03 1.489805752217892e-02  
2.556709294706036e-04 1.216248868687749e-03]  
[-3.324784208654945e-02 -5.783278081067757e-02  
-3.560895538219546e-02 -5.680073162233067e-02  
-1.174169201562238e-02 1.185578178858713e-01  
4.102433287299248e-02 1.323955590013154e-01  
1.346186724407323e-02 2.287233651551844e-02  
-8.792641635363215e-02 -1.719304585910407e-02]  
[-8.967853490280031e-02 -5.390194464941681e-02  
-8.606334021394316e-02 -1.697092655488963e-02  
7.637928428186860e-01 1.585195439271545e-01  
9.111151796214825e-02 4.256796627165119e-02  
-2.556814122777153e-02 -5.870376282541837e-02  
2.197199024177962e-02 5.790336582310560e-02]  
[1.435249488764887e-01 -8.202390015210534e-02  
6.089001507506192e-02 4.943543781173297e-02  
-1.164769440513463e-02 8.967643921756210e-03  
1.923303094581377e-02 5.274505098880270e-03  
3.141232241199606e-03 -6.796199303111142e-03  
-2.387254296073952e-03 5.019399556799832e-03]  
[1.196405783511569e-02 -2.222373189123121e-03  
-6.561309571872169e-01 -9.889372152388809e-02  
-4.112509867891259e-02 4.087791125230597e-02  
-2.570112944301553e-02 -8.005429583273591e-02  
2.940809951009440e-02 -7.327547093630286e-02  
-7.503580200105585e-02 2.696500723157646e-02]  
[-5.760313577293238e-02 2.283851034761798e-02  
2.965420880144480e-02 4.246427568794198e-02  
-5.582998095052196e-02 2.091177805774269e-02  
-7.676777205796383e-02 2.336354464749826e-02  
3.142820182629007e-02 7.084358692676139e-02  
7.993158587538264e-01 -1.783839505443735e-01]  
[-1.305746163103679e-02 -7.046452714522736e-02  
1.989843265928018e-02 -1.586203990232826e-02  
7.798840784613600e-02 -3.174737556186303e-03  
7.667775553311432e-02 -1.889064737959500e-01  
7.910129808748539e-02 5.292049694170580e-02  
1.317252995193481e-01 4.240448287367330e-01]  
[3.974535611072969e-02 8.873547432857665e-02  
4.875566389016674e-02 4.943760514018920e-02  
-4.985819439135913e-02 3.563579115979010e-03  
-3.842617472490292e-02 5.044897860084246e-02  
-8.884427161673375e-02 2.250448645442080e-02  
8.668631882367729e-01 2.567404570105574e-01]  
[1.234214151991417e-01 -8.107520145927017e-03  
1.481434932065346e-01 4.870706119773043e-02  
-9.219158144754167e-03 1.451900756134227e-02  
2.530358472162463e-02 -1.692955760150236e-02  
-2.756280337484944e-03 7.846225949029579e-03  
9.707050508558959e-03 1.691263867871555e-02]

[7.292839892929748e-02 4.761508428908613e-02  
 -2.824733550645493e-03 5.104238319451598e-02  
 1.314677150875615e-01 1.956730517298553e-01  
 1.018483551160780e-01 -1.805913088900121e-02  
 -2.100974339321765e-01 -4.630255294734821e-02  
 -7.015560428721891e-02 5.168995232256191e-02]  
 [-1.279216786555550e-01 -5.767822257171831e-02  
 -1.070935896744803e-01 -8.480443324348491e-02  
 1.482413600459714e-02 -3.887497038944041e-02  
 7.348098065528733e-03 2.776933746195089e-02  
 8.601471904807759e-03 -1.465175684414524e-02  
 2.310718724105602e-02 1.496619253341425e-04]

23

[1.444837754070339e-02 7.879476362386743e-02  
 3.992528460507837e-02 4.416978382893103e-02  
 1.287760294200562e-02 6.871447858922218e-04  
 2.047934580448719e-02 -4.703731195291225e-02  
 -9.223710567229154e-02 1.022927001331439e-01  
 1.123183649192607e+00 2.144662288251183e-01]  
 [4.600509766289074e-02 1.229281373701580e-01  
 5.126589032332755e-02 6.279597464890650e-02  
 -1.492260051186516e-02 -6.697180611156175e-03  
 -3.867101513775635e-02 1.369658061017222e-02  
 8.545811878047295e-03 5.626832027534254e-03  
 1.548663240816677e-01 -1.201965538971557e-01]  
 [-5.811933633376541e-03 -7.712200010265877e-02  
 3.084680257776020e-02 -8.602860040810231e-02  
 1.175411926044047e-01 1.128444108286062e-01  
 7.204059724142671e-02 -1.923269285607230e-02  
 4.135011715256471e-02 -4.638832122790725e-02  
 6.736447637480712e-02 7.199866001136204e-02]  
 [1.191563567368430e-02 -2.250579617992725e-03  
 -6.559872930591926e-01 -9.876753683420586e-02  
 -4.123234287443813e-02 4.089969317060349e-02  
 -2.561728971183417e-02 -8.015767298687618e-02  
 2.950475043025737e-02 -7.335904381635595e-02  
 -7.515228747147501e-02 2.692964163561546e-02]  
 [4.065587716116068e-02 -7.419822897550134e-02  
 4.434227380767512e-02 -2.850057809031369e-02  
 -1.847210661276336e-01 -1.426047611169938e-01  
 -8.576460094404702e-02 1.698570954976483e-01  
 1.167198697032202e-01 9.246844513169051e-03  
 3.564656233368741e-02 -1.004595170660480e-01]  
 [-5.544822667523043e-02 3.052094195468071e-02  
 3.680858612135312e-02 3.628886980882488e-02  
 -5.759673763058169e-03 6.587483281314370e-03  
 -5.778518102764810e-02 -2.901355611319257e-02  
 -7.913212903283246e-03 7.014608112409937e-02  
 7.317425245625632e-01 3.038494477823185e-01]

[4.460891467951777e-02 3.361671067600498e-02  
 -3.360250790697256e-02 2.890186448022927e-02  
 1.620532284898358e-01 1.404932535158385e-01  
 2.715813945106674e-02 -1.239028358666426e-01  
 -1.898875022322129e-01 -9.971051462250250e-03  
 -3.292547854593259e-02 3.387668037717017e-03]  
 [-4.302740010245208e-02 -6.343295580218168e-02  
 1.555757755224367e-02 -2.639083875198102e-02  
 -1.452667246206158e-01 2.593125150562638e-01  
 2.448029977947382e-01 5.045406160278362e-04  
 -1.103916231668675e-02 3.521836250288349e-02  
 -4.349821170821077e-01 1.342408803154768e-01]  
 [1.026056835738905e-01 7.404780379365634e-02  
 2.522561017075352e-02 1.109968758414154e-01  
 2.728692753405101e-02 3.073553542958555e-02  
 -2.487352442038353e-02 2.418649586053581e-02  
 -4.012201883962880e-02 -2.068704468682612e-02  
 -3.189918415602437e-02 -1.962234398068906e-03]  
 [-9.068659635622264e-02 -5.336224145680598e-02  
 -8.454281600928386e-02 -2.364343841031450e-02  
 8.739217149983684e-01 6.798685205387187e-02  
 6.610564636247716e-02 7.498359356972366e-02  
 -1.075277534258647e-02 -7.998221952419775e-02  
 7.964548254691420e-02 1.128799767385239e-01]  
 [-6.580738620367620e-02 2.357316056496507e-01  
 -2.659099846586309e-01 -2.628889958863644e-01  
 2.045758686163050e-05 4.399812693891360e-05  
 2.454066371924251e-05 -2.379020137399010e-04  
 -6.144454008688954e-05 1.230786999647136e-05  
 -4.878334387465467e-05 -6.963423426514792e-05]

24

[-2.890387266144671e-02 -4.970534199564261e-02  
 -9.027219428993132e-03 -9.390152527846693e-02  
 6.058750122708433e-04 9.184287005957571e-03  
 -2.738574220012846e-03 8.035397716732201e-02  
 8.501691288475255e-02 1.485407984462131e-02  
 3.599271065112269e-02 4.231113238199435e-02]  
 [1.277218866909036e-01 6.829922237085212e-04  
 -1.005133234978212e-02 -8.998040370460270e-02  
 -2.625316096340404e-04 -7.311441732646040e-04  
 -1.190481574284817e-04 -7.439634349408870e-04  
 7.054617716325696e-04 -2.749691919369806e-04  
 -2.672939518820095e-04 7.588112962492389e-04]  
 [-9.140845105789551e-02 -5.232423892026299e-02  
 -8.774013265879121e-02 -2.150790879616284e-02  
 8.095490422803700e-01 1.037101592132614e-01  
 7.738198826132098e-02 8.702807592461556e-02  
 -8.332260958462405e-04 -6.572580824905035e-02  
 4.890192758751384e-02 9.313989753745242e-02]



[-1.999995412615886e-02 -9.748041627783154e-02  
 3.210060282610028e-02 -1.882893724839837e-02  
 6.371352495841011e-02 2.906260731959327e-02  
 1.811875662666422e-02 -8.105943611395500e-02  
 -3.768206864562610e-03 2.791207726437486e-02  
 -1.178967550550229e-02 1.401264279335293e-01]  
 [-5.688851238087889e-02 2.607754395636174e-02  
 3.170529095630332e-02 4.286640687400977e-02  
 -4.780259340096224e-02 -3.144552509261566e-02  
 -1.102013108034954e-01 3.719808756810113e-02  
 1.692811501194303e-02 8.832011121834717e-02  
 7.644191786660300e-01 -8.504729026081359e-02]  
 [1.195828093580672e-02 -2.226637866891123e-03  
 -6.560431908124870e-01 -9.891087029248244e-02  
 -4.116142999025663e-02 4.092184461506645e-02  
 -2.570881662550588e-02 -8.006441970725052e-02  
 2.942538204725383e-02 -7.333140736206359e-02  
 -7.507820573963410e-02 2.699787994888321e-02]  
 [8.881119649521659e-02 2.574237749218361e-02  
 6.825273665753507e-03 4.426177954663865e-02  
 1.618845675470742e-01 1.726260087969597e-01  
 8.052380111333796e-02 -1.631321068752367e-01  
 -1.792383374112605e-01 -3.204187922551609e-02  
 1.977162267701838e-02 -2.028668197342480e-02]  
 [8.378734907266165e-02 7.086999354310029e-02  
 2.831717418651807e-03 6.184797891728196e-02  
 -4.711578295593539e-02 7.366671905947451e-02  
 7.280032352251421e-02 1.279964254447864e-01  
 -4.354548214161386e-02 -6.097430492772671e-02  
 -4.041221465878353e-02 7.059805743572223e-02]  
 [-4.606391038626012e-02 -1.040875826404035e-01  
 2.143206158505825e-02 -1.038194176101155e-01  
 1.371269314270939e-02 5.644779052512083e-02  
 2.835347962539606e-02 -3.131700006235745e-02  
 -7.110364315732441e-03 3.394105567332519e-02  
 -4.233481981952896e-02 5.308444537848198e-02]  
 [3.702632212815336e-02 8.947777913499096e-02  
 4.903290825518159e-02 4.803735232898403e-02  
 -3.474424732489185e-02 -4.535165369209423e-02  
 -1.137761776913837e-01 8.019812092616779e-02  
 -8.807433795712825e-02 3.398393264831444e-02  
 8.302417338503350e-01 1.807764403581605e-01]  
 [4.768789125350240e-02 1.613857801148282e-02  
 7.508645238629058e-02 3.117554119850644e-02  
 -7.658040140123829e-02 1.021978509433057e-01  
 1.732652344248390e-01 -7.281142647258017e-02  
 3.460141038787490e-02 2.549255976059995e-02  
 8.799620473614307e-02 1.426054437143593e-01]

[7.945250609473577e-02 -3.127155783262247e-02  
1.521322912569005e-02 2.730045186909798e-02  
-4.858136794362269e-02 8.429754295012977e-03  
1.009016232211789e-01 -6.314103498177542e-02  
8.819770196977672e-02 -3.515430181510248e-02  
6.966876688422236e-02 5.075488113632681e-02]  
[5.920417816570048e-02 -9.393773701614571e-03  
8.643005705160457e-02 2.512611143071384e-02  
-6.424489107986232e-02 7.578371606714206e-02  
1.285476195909422e-01 -3.200797441960745e-02  
-2.010096817415938e-03 1.770980112765704e-03  
5.166251122940563e-02 1.167807839673655e-01]  
[-1.170910152691182e-02 -8.675662784553030e-02  
2.141579907606376e-02 -2.784714349227905e-02  
1.885669122324491e-01 7.543961609540960e-03  
2.200096949315476e-02 -2.221762579894826e-01  
5.664190492798248e-02 7.332071157644089e-02  
1.295204533111596e-01 3.184341659827840e-01]  
[1.196987437518895e-02 -2.214313709739025e-03  
-6.561206531480615e-01 -9.891808804360983e-02  
-4.113175093131811e-02 4.090072920970762e-02  
-2.570028607543965e-02 -8.002682129694531e-02  
2.940672666204226e-02 -7.329841511857396e-02  
-7.503049407166659e-02 2.698282543009154e-02]  
[-5.854393833693551e-02 2.209375034507742e-02  
2.932153708218600e-02 4.153295261943363e-02  
-5.080317045192330e-02 -1.344539638450755e-02  
-1.032854890312835e-01 3.373236316367239e-02  
3.987256318064245e-02 8.641268872287346e-02  
7.709352119514280e-01 -1.831241134686611e-01]  
[-5.277980261190859e-02 -3.434267934171099e-02  
-2.854021854494327e-02 -9.480330652358518e-02  
-1.920602273987353e-02 -8.383456139662366e-03  
-9.105834251135201e-03 7.488896827391686e-02  
4.481192422293255e-02 -3.271987707835900e-03  
1.651539355676153e-02 -5.971403868292191e-03]  
[-9.184760294862220e-02 -5.225552135790038e-02  
-8.955686440547454e-02 -1.945544567776849e-02  
7.607984957743145e-01 9.243677911183532e-02  
6.456983924969004e-02 8.222090488485802e-02  
-4.130022028134782e-04 -6.213341590706173e-02  
6.411075674066288e-02 6.970248064094375e-02]  
[4.022094496015276e-02 8.880860430074865e-02  
4.872057624878511e-02 4.942440556136371e-02  
-4.198427804903931e-02 -3.161948687918655e-02  
-7.761219546818308e-02 5.012382764798609e-02  
-7.619624040166494e-02 3.778992529470857e-02  
8.485510200211286e-01 2.566625679460031e-01]  
[-2.154304550012626e-02 -1.318951231643573e-01  
1.917525962141841e-02 -1.660981447435979e-01

-6.410049744171748e-03 8.950892416492868e-03  
 1.618117441616143e-03 2.063188581716270e-03  
 8.753381418961368e-03 8.779986671068081e-03  
 -6.292299521926412e-03 8.050088093155139e-03]  
 [1.051210127470124e-02 2.079592648430709e-03  
 -2.979598500125295e-02 1.712633477014691e-02  
 -1.720844930403869e-01 2.693516092044525e-01  
 -7.758958141657615e-02 1.583902568001637e-01  
 -1.238275532945082e-01 -1.819115688489588e-01  
 -2.212011825573485e-01 -2.252584048987643e-01]  
 [4.246830555607955e-02 4.929821874206852e-02  
 -1.853092778440245e-02 5.464482218703159e-02  
 2.968793322313505e-01 6.033984200993699e-02  
 1.735548733222815e-01 -2.042108629983036e-02  
 -2.211299823486222e-01 1.398508444729653e-01  
 -3.099896905099526e-02 2.120506927896417e-01]

26

[-2.318697576964488e-02 -1.336519454502662e-01  
 3.002505461369349e-02 -7.869391704370217e-02  
 7.973231522799898e-02 2.372093960446784e-02  
 -2.052707347640676e-02 -9.473921230869219e-02  
 7.845658362954514e-03 4.099874252291313e-02  
 8.948206449913634e-03 8.388124668175320e-02]  
 [4.883115973753014e-02 9.557113978474562e-02  
 5.128196750223744e-02 5.041973950423439e-02  
 -1.067184269962287e-02 -1.801934245929761e-02  
 -8.558228048119838e-02 -1.126445999399861e-02  
 -4.286189410258511e-02 -5.747796168850071e-03  
 5.463795835212959e-01 2.201676263250207e-01]  
 [-7.435445357673245e-02 1.019429565743096e-02  
 2.782517384007864e-02 4.371152796063806e-02  
 -3.200622216653090e-02 -2.695100420255106e-03  
 -6.105012643388731e-02 6.583775590861904e-02  
 3.082037140801959e-02 3.183277704325802e-02  
 3.119572467549174e-01 -2.662670798709086e-01]  
 [4.649054215284048e-02 -1.993447367109604e-02  
 1.260546802734415e-01 3.981544789851258e-02  
 -5.001316897332229e-03 2.435080823232331e-02  
 2.023268979036831e-02 -3.018021686509676e-02  
 3.446362341858038e-03 4.377520596668926e-04  
 2.377752665329312e-02 1.909189764323990e-02]  
 [3.785556317164072e-02 -2.513384785996059e-02  
 -1.710773801221028e-02 -2.744526921970957e-02  
 1.216446134156147e-01 7.478264719689032e-02  
 4.041399420410997e-02 -1.449020761602249e-01  
 -9.859464630544614e-02 2.925386803293134e-02  
 5.862340253935415e-03 2.322868629581595e-02]  
 [8.941378268050428e-02 3.892921402300804e-02  
 1.641330382667569e-02 5.970791479162590e-02

4.735283267010847e-02 1.977170790982055e-01  
3.641764079166517e-02 2.854026965935670e-02  
-1.589573464573369e-01 -1.444931295127709e-01  
-8.335422814880138e-02 -5.114276746240517e-03]  
[1.227399568349182e-01 4.779110747214089e-01  
-9.863144540417489e-02 2.871290377371253e-01  
-3.801684922188757e-05 1.572205001623818e-04  
3.358481041429982e-04 2.079011895695168e-04  
-1.203995212344968e-04 -1.525857477381404e-04  
1.157335641631757e-05 7.725339884147905e-05]  
[-9.249083719022291e-03 -6.377050867095604e-02  
-7.706437437501829e-04 -8.490071069887671e-02  
-9.739288618211650e-02 3.597973222479823e-02  
5.722550201708212e-02 1.782023439715127e-01  
1.060854068879202e-01 -3.762472309007240e-03  
-3.520199074608151e-02 2.387664638436500e-02]  
[-9.095163006588077e-02 -5.335433047478313e-02  
-8.692157210629790e-02 -2.099609626637079e-02  
8.168113992027339e-01 9.877968770433525e-02  
6.784884069661723e-02 8.622161343335467e-02  
6.327754970180195e-03 -6.171163908987549e-02  
3.835295808734283e-02 9.888822278851314e-02]  
[1.196618373296718e-02 -2.226525393279340e-03  
-6.561243241323272e-01 -9.876727333494066e-02  
-4.116867028629848e-02 4.085826962498781e-02  
-2.564483494859406e-02 -8.004899709862651e-02  
2.948371041755447e-02 -7.327455141346406e-02  
-7.507420614531009e-02 2.690271792338620e-02]  
[1.101525342003926e-02 2.988833819305047e-02  
4.103518072769424e-02 3.712425295194478e-02  
-7.746348917741691e-02 3.465700321414725e-02  
1.682294558123468e-01 -1.422858737110154e-02  
-3.936765068457141e-02 1.787744820362256e-01  
8.757821584559102e-01 4.203316229268079e-01]

27

[6.816481270031778e-02 3.770282669371593e-02  
-1.091484590279539e-02 5.569316061330906e-02  
9.610159271729109e-02 2.487621613105041e-01  
6.526193191689847e-02 -5.530873267605956e-02  
-2.152483690751999e-01 -1.290221295129843e-01  
-8.348257212129531e-02 4.295802479144411e-04]  
[-3.635969653013102e-02 -6.743535340244054e-02  
-3.532508153602856e-02 -4.108510652664332e-02  
-2.281109158958908e-01 -7.874374711238018e-02  
-4.660694313450896e-02 8.850100163350086e-02  
2.576638456024759e-04 5.664570611615515e-02  
-4.507290335990216e-02 -8.157777610912437e-03]  
[-5.691155821044424e-03 -6.083872678712002e-02  
4.841069655528670e-02 -4.446907106762750e-03]

6.338231752693534e-03 2.485627874326435e-01  
 3.754087211522099e-01 -1.962535650591449e-01  
 -4.519412502359963e-02 4.331306920761118e-02  
 -2.098222504520704e-01 5.342729072572187e-01]  
 [2.122429806889772e-01 1.448766082490933e+00  
 -1.224262136873884e+00 7.488924472748163e-01  
 -1.298255539116598e-06 3.347496869012925e-07  
 2.108795564626654e-06 1.195821181627323e-06  
 2.681656773096877e-07 -9.679649503947570e-07  
 6.307207034032863e-08 5.418115364127808e-08]  
 [1.195207417998484e-02 -2.215428835938167e-03  
 -6.561295176314568e-01 -9.885102380229383e-02  
 -4.115614898414911e-02 4.089525146806702e-02  
 -2.566859401291105e-02 -8.006176387899371e-02  
 2.943591277380081e-02 -7.329732907950910e-02  
 -7.505226447181940e-02 2.694585086480025e-02]  
 [-2.276181721029983e-02 -8.482616535446122e-02  
 3.483748217481483e-02 -1.223616505553305e-01  
 6.498035088179047e-03 -1.030550951125800e-02  
 2.218430082874905e-02 4.676091336668773e-02  
 3.985207851252954e-02 -1.937705223281217e-02  
 1.575092393287295e-02 6.449221151616088e-03]  
 [3.964860910396011e-02 9.051448446659485e-02  
 4.906323494402534e-02 4.869511005926710e-02  
 -3.249766387224527e-02 -1.725908350367700e-02  
 -5.412476461656217e-02 1.764588364974175e-02  
 -6.303519316713262e-02 3.317508596643876e-02  
 8.313780794926317e-01 1.977151261751709e-01]  
 [3.124391893518505e-02 5.709548358231878e-02  
 -5.870291011031855e-03 9.874405849988363e-02  
 2.964655948750937e-02 -3.429380244803087e-02  
 3.576698996245281e-02 5.207701834960840e-02  
 -8.750491392065256e-03 4.405770628244204e-02  
 1.343398752424562e-02 5.502472101290749e-02]  
 [2.116494200105904e-02 -1.227747052796779e-01  
 9.224113686004103e-02 -5.873095236840039e-02  
 6.905598287578828e-02 -8.781545357375248e-02  
 -1.376364109157576e-01 1.798131912524833e-02  
 3.631491522690449e-02 1.582950705986736e-02  
 7.571829812949882e-02 -3.513479509681663e-02]  
 [-8.674340811890308e-02 -4.964627604418618e-02  
 -8.287894403193623e-02 -1.863948343441149e-02  
 9.274085781449244e-01 2.192374770907845e-01  
 1.044423193103900e-01 1.006789100756603e-01  
 1.288287116707382e-02 -8.086835604122318e-02  
 6.172808044511442e-02 1.134166213319330e-01]  
 [-5.008943481948743e-02 1.805087640012419e-02  
 3.293215922259706e-02 3.924307174068851e-02  
 -3.148423680064527e-02 -1.875147138182239e-02  
 -1.411300032102792e-01 -8.375846042758730e-03

5.759179628372209e-02 1.017002076522537e-01  
1.032861726301485e+00 -2.458969457643913e-01]

28

[-9.160376401737276e-02 -5.232486923504314e-02  
-8.800951078661762e-02 -2.140745194689663e-02  
8.050844686804359e-01 1.029788633697507e-01  
7.570351124981749e-02 8.577924860699614e-02  
-1.060105105446654e-03 -6.534855184259590e-02  
4.940602145976548e-02 9.266434975467970e-02]  
[8.325945088719254e-02 6.910468218913836e-02  
-3.356690527067312e-05 6.599964927638415e-02  
-3.364444828757073e-02 7.862499123556085e-02  
6.534036304108899e-02 1.080202933826855e-01  
-4.584982065656690e-02 -7.003545414727079e-02  
-5.006469721600093e-02 8.646987622318501e-02]  
[-3.392984246732750e-02 -1.025927644077751e-01  
2.336070402269936e-02 -9.258952374370852e-02  
3.949365589048949e-02 7.231685443318610e-02  
3.196826088607856e-02 -5.081696016877967e-02  
-2.053309700917965e-04 4.888782224487572e-02  
-4.266843770650746e-02 9.082045023868847e-02]  
[5.512797434525198e-02 1.464376790207130e-02  
8.667004027676127e-02 3.411080915858548e-02  
-4.300180221249737e-02 6.397042340912312e-02  
9.673844503677682e-02 -5.719426582259336e-02  
4.149488786689420e-02 1.333460432108252e-02  
5.289167506231885e-02 4.259588491730266e-02]  
[-4.432892659305141e-02 -9.388102235375667e-02  
1.808096320477865e-02 -8.621864860722016e-03  
3.448221369682043e-02 3.815222095274983e-02  
4.231903990935702e-02 -4.695413744770727e-02  
-8.425599265138285e-03 1.060299715127737e-02  
-7.453727112105943e-02 8.232926075342111e-02]  
[8.945477383876128e-02 2.480131592364506e-02  
3.123383262107739e-03 4.571429626107529e-02  
6.210252772090904e-02 1.219779483136850e-01  
6.726821321715783e-02 -6.494501824145262e-02  
-1.025620684092608e-01 -4.196753509457529e-02  
-1.698984351955730e-02 -1.075634481940440e-01]  
[-2.973961695974477e-02 -4.781431878778445e-02  
-7.533050465855908e-03 -9.335400317226728e-02  
-9.890561216672903e-03 -4.254357178172213e-03  
-1.462305375330421e-03 8.883453786512312e-02  
8.240169295650635e-02 6.767067910599364e-03  
3.994548054017034e-02 2.405907880503144e-02]  
[1.195481223296774e-02 -2.226362013003683e-03  
-6.560680958515093e-01 -9.891915070142685e-02  
-4.115143647298693e-02 4.091869460333655e-02  
-2.570836417365118e-02 -8.005259640653499e-02

2.941647670336166e-02 -7.332220659943245e-02  
 -7.506358428275917e-02 2.699531454264606e-02]  
 [3.216634984290338e-02 8.914340214501186e-02  
 4.957200362557210e-02 4.881077346220454e-02  
 -4.124794929424990e-02 -2.708100660937866e-02  
 -8.188238390774597e-02 7.974016042874993e-02  
 -7.731417448796273e-02 6.410555342843209e-02  
 9.272569613284856e-01 6.398496674517834e-02]  
 [-5.223626464400074e-02 3.564402293390440e-02  
 3.404203267339312e-02 4.504469239178039e-02  
 -3.791900826204594e-02 -2.595219293473410e-02  
 -9.774518412706094e-02 -1.310250056416336e-03  
 -1.231434497255368e-02 9.713030796868173e-02  
 7.955271866812232e-01 1.510103699351196e-01]  
 [9.675532731130372e-02 1.982614555020259e-02  
 1.938460751697549e-02 5.529632100200375e-02  
 6.749105601528511e-02 4.863650492565792e-02  
 2.536006031975780e-02 -7.745467777539833e-02  
 -6.147428634242829e-02 2.000842112214775e-03  
 1.173767726675300e-02 9.169846002938607e-02]

29

[2.202278355124121e-02 1.865027065415976e-01  
 -2.226139651142897e-02 1.387982161703928e-01  
 4.923594511902486e-04 7.195878336589201e-03  
 7.032974862145538e-03 -2.358026833522016e-03  
 -3.159740287831742e-03 -7.430292853718858e-04  
 -2.534180976241952e-04 1.799687029314703e-03]  
 [7.527097133508774e-02 4.333708878036806e-02  
 -4.077104923273455e-03 5.446378522504745e-02  
 1.631934428026570e-01 1.854084804163748e-01  
 1.664126209938336e-02 -3.717485425148249e-02  
 -2.031626672666073e-01 -4.365655681971344e-02  
 -8.012023801156498e-02 2.082688850367845e-02]  
 [-9.596419311598827e-03 1.843001785692495e-02  
 -6.378165743252558e-02 9.496733018236014e-03  
 -3.040373048053669e-02 6.255483549071883e-02  
 5.534773219853462e-02 -9.120946563870576e-02  
 -5.944661472349186e-02 -2.823410532907225e-02  
 1.639232429046954e-02 -4.060359998811391e-02]  
 [-5.360708332665898e-02 3.203736058863828e-02  
 3.248699108558692e-02 4.022983313968830e-02  
 -5.600146717891284e-02 8.905408414392177e-03  
 -9.071142416543220e-02 -4.086288532708761e-03  
 5.931949618279434e-03 9.442843740082266e-02  
 8.579835438943437e-01 8.517059574989552e-02]  
 [-4.012313976796235e-02 -9.491163399767721e-02  
 1.871763040984198e-02 -4.403803031947792e-02  
 1.045744443445821e-01 8.066679757062953e-02  
 8.782456932830295e-02 -1.551569183021007e-01]

-3.074460030620818e-02 4.845455675075255e-02  
 -1.116028544188805e-01 1.759018380321524e-01]  
 [1.194466370578808e-02 -2.227934256287035e-03  
 -6.559814680895214e-01 -9.884016457468742e-02  
 -4.118365455628449e-02 4.093834378515152e-02  
 -2.568055618670353e-02 -8.010022961694104e-02  
 2.947058311147348e-02 -7.336753984306756e-02  
 -7.513099025087204e-02 2.698124311269894e-02]  
 [3.539469566131193e-02 9.052072774963449e-02  
 4.724932326760357e-02 4.917035063328780e-02  
 -1.886232526657566e-02 -1.674874568651438e-03  
 -6.374348022906246e-02 2.865728855691004e-02  
 -7.706207654382645e-02 5.429159735705216e-02  
 9.304246068173611e-01 1.357686724635740e-01]  
 [-5.797186816762868e-04 -5.273168322768926e-02  
 1.304173302051314e-02 -5.180834512420517e-02  
 -6.680081520923058e-02 3.743503380368757e-02  
 1.348779489237379e-01 2.155061353330062e-01  
 1.752694514185229e-01 -8.125470419700284e-04  
 3.366828369704720e-02 1.177715949882861e-01]  
 [9.562051936236410e-02 -4.246480706729051e-02  
 1.460096606630596e-01 -8.735925259970513e-04  
 -2.847534902923765e-02 -5.866781012212931e-03  
 2.178758403284134e-02 2.159461944135132e-02  
 8.593336956320177e-04 1.087831631568330e-02  
 -1.355195230185147e-02 1.807826722378871e-02]  
 [-2.188620414723062e-01 -1.134810548651070e-02  
 9.695603725032541e-02 -3.571102967642476e-02  
 6.301068853349905e-04 -9.080986077365250e-04  
 -7.242261913525560e-04 -1.034112350917995e-03  
 -2.854208568500995e-04 3.330971230031213e-04  
 -7.587457740463062e-05 8.988720459771171e-04]  
 [-9.180345190431878e-02 -5.138241890063549e-02  
 -9.039787348054081e-02 -1.957568045893779e-02  
 7.746357044949297e-01 9.563392089182210e-02  
 5.524727140385109e-02 8.900818655978317e-02  
 6.437129458220735e-03 -6.941677917482944e-02  
 5.970773745180848e-02 1.024705045893424e-01]

30

[2.953578525527156e-01 8.546651922231188e-02  
 -7.346643179447110e-02 3.073798100920773e-02  
 1.662317698836563e-04 -4.319305202672735e-04  
 -4.606058592410838e-04 -1.417929487740936e-04  
 2.978010299800752e-05 1.490715949362021e-04  
 -2.468390602399686e-04 -5.385243855479885e-05]  
 [1.195047909112391e-02 -2.235598374365038e-03  
 -6.560622371322551e-01 -9.889894801358151e-02  
 -4.116922538066388e-02 4.092087609145028e-02  
 -2.569505049083936e-02 -8.005244624673852e-02



2.943399043125658e-02 -7.332474230211750e-02  
 -7.507338376507336e-02 2.698505960056657e-02]  
 [8.206907441767480e-02 3.939433389303309e-02  
 9.379268992812949e-02 6.601763016425209e-02  
 8.307679364228953e-03 4.046209371942824e-02  
 3.806066933308012e-03 -6.372453915028789e-02  
 2.267301911173887e-02 -1.677516936297290e-03  
 5.247059330047904e-02 -2.865338681233276e-03]  
 [-9.062004874923041e-02 -5.368111035933029e-02  
 -8.719912606249301e-02 -2.312781420499943e-02  
 8.347728608212008e-01 8.355054298978265e-02  
 9.245582939308021e-02 8.166253493167300e-02  
 -2.354214652484441e-03 -6.809755288168812e-02  
 4.814368500782844e-02 9.714777233839450e-02]  
 [3.504001802298350e-02 9.268155907411310e-02  
 4.790242694707059e-02 4.793995872260172e-02  
 -6.763199943261145e-02 -1.699707663080452e-03  
 -2.421781095265151e-02 7.935914924881782e-02  
 -7.759542458680944e-02 4.953338533412120e-02  
 8.651296890386153e-01 1.553277914816578e-01]  
 [-2.972510821146758e-02 -3.618140192017372e-02  
 -2.317199737516067e-02 -8.078755408929225e-02  
 -9.541378996069182e-03 -8.967937325053371e-04  
 -3.582999319679166e-02 9.268934846248260e-02  
 6.885286049579889e-02 4.090537844140373e-02  
 1.231440678035006e-02 3.749240659198565e-02]  
 [7.771748533712526e-02 5.302977694002348e-02  
 -6.155384547708565e-03 5.289165756104954e-02  
 7.419805379568593e-02 1.538454038340474e-01  
 1.093519659170811e-01 3.422275875118293e-02  
 -1.409181829595765e-01 -4.047499780795253e-02  
 -1.298459896960314e-02 4.709568176640969e-02]  
 [-5.098603121573841e-02 3.403952862110539e-02  
 3.452279064879247e-02 4.314457892072995e-02  
 -6.570595506940161e-02 -2.284936714231018e-02  
 -7.923925112776441e-02 8.581676336689624e-03  
 -2.483088216492673e-03 1.018552264594977e-01  
 8.412873341140910e-01 1.292192153025627e-01]  
 [-4.529733943589832e-02 -1.053810077783712e-01  
 -2.115877496090988e-03 -8.617679657666251e-02  
 4.331070282047361e-03 1.144160390737479e-01  
 6.790934673338343e-02 -1.031660405454535e-02  
 -1.136875391311876e-02 3.540444304967277e-02  
 -9.264535705957309e-02 4.794975046157596e-02]  
 [-3.876769385806253e-02 -9.046789408865608e-02  
 1.764846563708608e-03 -8.487589675362709e-03  
 4.719874924584731e-02 2.482233379152294e-03  
 7.306473717486877e-03 -7.722866948667306e-02  
 5.767349821036541e-03 1.346376392373291e-02  
 -1.565365019417942e-02 1.253705201296453e-01]

[8.771787313180120e-02 -8.826536886661711e-03  
2.621892846935486e-02 3.861051069375650e-02  
1.687262985776816e-02 1.004895544913193e-01  
8.251268500919445e-02 -8.140508147915494e-02  
-4.793000831703392e-02 -6.558101142201993e-02  
-5.300710699863117e-03 -1.860444280241580e-02]

31

[-3.694210660529709e-02 1.275608510773267e-02  
-9.121636417555813e-02 1.800507430370951e-02  
-6.597402491632952e-02 2.742761934349562e-02  
7.050620322940284e-03 -5.373031879872089e-02  
-2.624877563775423e-02 -1.066771381102895e-02  
-1.469165341319217e-02 -8.267117597444532e-02]  
[-9.114098778619215e-02 -4.903994326008500e-02  
-9.268632866120284e-02 -1.472665642522166e-02  
7.395287851631415e-01 1.239154701767779e-01  
5.233757873273089e-02 1.044288249296829e-01  
4.186016617493228e-03 -7.640824421967769e-02  
1.021058568534401e-01 9.343985286650186e-02]  
[6.451014935533699e-02 4.680952670733235e-02  
-9.107681087212395e-03 5.560721194337961e-02  
1.496752287172783e-01 2.007931453203014e-01  
6.442638982397526e-02 1.569956118037822e-02  
-2.164981658899957e-01 -4.648634959725002e-02  
-1.073237199854112e-01 5.555038346423834e-02]  
[-2.698000366857724e-02 -4.356919006588061e-02  
5.312576046727510e-03 -4.056595694021779e-02  
-4.714705427336187e-02 -5.908197038742778e-02  
4.044137378833949e-02 2.910145242235341e-01  
1.735008655020513e-01 -3.531432677824800e-02  
1.866506659569952e-01 -7.628483453644913e-02]  
[1.065025684893787e-01 -3.627047823308294e-02  
5.716700997528990e-02 2.448174264952370e-02  
-2.206331214956215e-02 4.977842031259672e-02  
6.693247620329199e-02 -1.269641281708275e-02  
3.294269863363656e-03 -2.988840727433806e-02  
1.450492916534533e-03 2.117597562736541e-02]  
[-6.807503498592023e-02 -1.405126660149260e-01  
2.423907761654835e-01 2.037364863160492e-01  
3.070216983118614e-06 2.548724423949297e-04  
5.115814436570941e-04 1.397344024318265e-04  
1.482350422244082e-04 -1.127600339883129e-04  
-1.145697772159959e-04 2.088942114952030e-04]  
[1.389881941407869e-01 -2.306960640063502e-01  
2.297811510692723e-01 -2.073597290146669e-01  
2.131045930063957e-03 -5.433118940914990e-04  
-1.400317773309300e-03 -3.845491487689927e-04  
3.869499619885019e-05 -8.916562636870682e-04  
5.591551920253446e-04 -4.582042140627516e-04]

[1.192616685154720e-02 -2.195936002846045e-03  
-6.559681872918294e-01 -9.919345885964885e-02  
-4.107454200222341e-02 4.103126084856650e-02  
-2.580180377093794e-02 -8.003441429107427e-02  
2.931581191637179e-02 -7.343604805323659e-02  
-7.503287007812516e-02 2.716822278656868e-02]  
[3.881646261118304e-02 9.077116512923165e-02  
4.899321455559123e-02 4.921082935841720e-02  
-3.498601415898454e-02 2.047605482018378e-03  
-5.604595275035771e-02 2.178853811188747e-02  
-6.716518474030780e-02 3.546324565382435e-02  
8.509729250628838e-01 1.713880376220182e-01]  
[-4.608454620761240e-02 2.369040595817177e-02  
3.357801163197605e-02 3.928002863170627e-02  
-4.975956006975440e-02 1.405313652088325e-02  
-1.202116909213986e-01 -4.682703847331243e-02  
2.693080887138527e-02 1.201208655709573e-01  
1.065980621397583e+00 1.994191558432812e-02]  
[-4.027296244464722e-02 -6.797128767084987e-02  
4.336768606782387e-03 -2.480689784613329e-02  
1.714650938006652e-01 1.106126963552498e-01  
1.696594009773146e-01 -2.557521149542831e-01  
-8.339524922371772e-02 1.097768422599622e-01  
-3.931157356326855e-01 4.156054963130359e-01]

32

[-5.976473478805180e-02 -5.711548296408651e-02  
-1.779828877203823e-02 -1.445261432870978e-02  
-3.393054169901837e-01 5.557169794408085e-01  
1.313052957321461e-01 2.957559284798357e-01  
-9.412945852000902e-02 -1.286269281736005e-02  
-3.132192641258906e-01 -6.918895150285542e-01]  
[9.276301702114380e-02 2.336527081631053e-02  
1.045383967744024e-02 4.520084364725709e-02  
1.561284715010618e-01 1.560320687879385e-01  
8.184575756733835e-02 -1.759000289473579e-01  
-1.664148834812526e-01 -2.256901174751832e-02  
2.645307610503609e-02 3.035443749575205e-02]  
[-9.200709083408552e-02 -5.538526935654002e-02  
-8.483118762680947e-02 -2.765865577531521e-02  
8.776675345862479e-01 -9.599905205733501e-02  
6.763338642081994e-02 5.829235719752276e-02  
8.958660873137540e-03 -7.856214929760086e-02  
8.945569584462805e-02 1.407762000368563e-01]  
[-7.130344346633495e-02 1.544392205336172e-02  
2.321673066769402e-02 4.876474570447829e-02  
-1.565336655786206e-02 3.387895424743942e-02  
-4.183313717546787e-02 8.316065355779848e-02  
3.969786962419326e-02 4.368355696408954e-02  
3.759155207793492e-01 -4.133934500642211e-01]

[-1.547566603010366e-02 -4.924496831802056e-02  
 -1.367715423193744e-02 -5.708045470445464e-02  
 -1.936238878285178e-02 1.970869906915351e-01  
 1.709253773486542e-01 2.154398639086723e-01  
 4.486294240416146e-02 4.076684478754161e-04  
 -1.720844615248495e-01 2.151550043144367e-02]  
 [-2.341066773938693e-02 -5.349695859176813e-02  
 1.390383625640628e-02 -1.344794897379776e-02  
 3.245236984559453e-01 -4.505729188041678e-01  
 -2.625696016105848e-01 -5.860254977540074e-01  
 1.514888278062248e-01 1.066951666923373e-01  
 9.867922597414897e-01 9.716263946725927e-01]  
 [1.196767722724355e-02 -2.233674380995585e-03  
 -6.561275830418958e-01 -9.885783387916217e-02  
 -4.115647121360864e-02 4.086681222773998e-02  
 -2.567273050604941e-02 -8.003472954236912e-02  
 2.944789340691421e-02 -7.327618267678629e-02  
 -7.504795452149145e-02 2.694548550501042e-02]  
 [5.635854202647309e-02 -4.438685404702911e-03  
 8.853236472008040e-02 1.820810991734960e-02  
 -6.652550861317332e-02 6.032974127503370e-02  
 1.672558198885781e-01 1.070769945248233e-02  
 -2.938598083906530e-02 4.600426366994089e-02  
 4.489585020947580e-03 2.235485088271092e-01]  
 [4.271659045666389e-02 8.927192186195841e-02  
 4.869742858100710e-02 5.040050733573848e-02  
 -3.715864267586455e-02 -2.300875018711463e-02  
 -1.025387300865895e-01 6.451870481071663e-02  
 -9.174942476699161e-02 6.653817359822764e-03  
 7.579064498245012e-01 2.862420015469492e-01]  
 [8.844161609101692e-02 6.737846896581375e-02  
 5.604316173884615e-03 6.055294297926491e-02  
 -4.396259865695284e-02 9.246001785776033e-02  
 8.201288895806473e-02 1.315287015059228e-01  
 -5.082978815547608e-02 -7.301772589448312e-02  
 -7.708182754357300e-02 3.376672678758898e-02]  
 [-2.392613976743667e-02 -3.509214417920490e-02  
 -5.388445119885423e-02 -8.424352406537047e-02  
 6.603405205157981e-03 -5.650189895887306e-02  
 -7.046467046066390e-02 -3.379731830454447e-02  
 2.160668965476390e-03 4.899873675297185e-02  
 1.386208889268512e-02 1.557227354006691e-02]

33

[1.149990744648977e-01 1.596886956746401e-02  
 1.754419743501118e-02 4.740812624889496e-02  
 3.782889309274285e-02 9.541285392547171e-02  
 2.437761296211938e-02 -4.739555364054290e-02  
 -7.669065243980261e-02 -5.184147137855603e-02  
 -8.906614485322361e-03 -7.428012464962150e-03]

[-3.029114404956101e-02 -1.046370726924797e-01  
 2.556169470991512e-02 -3.863400909769825e-02  
 1.058730825847461e-01 1.660029158357758e-02  
 1.738830164063688e-02 -9.786105966827846e-02  
 5.902143352578795e-03 7.179026604621215e-02  
 -3.449551275743423e-02 1.350994906730606e-01]  
 [-2.793890018721732e-03 -7.843810995035572e-02  
 4.226635316447041e-02 -8.469533273279803e-02  
 1.438557605981023e-02 5.313283495078121e-02  
 3.507712778182020e-02 -4.485839146883738e-02  
 7.651637517974681e-02 -4.554650307010322e-02  
 8.198978729089806e-02 9.739479506049463e-02]  
 [-9.221163016906142e-02 -5.304459783142781e-02  
 -8.940252165354032e-02 -2.211163762769012e-02  
 7.750322087092483e-01 6.129047294328547e-02  
 6.570347105437757e-02 8.824264951748027e-02  
 1.118698525367483e-02 -6.005730593090031e-02  
 5.871662158134940e-02 8.003056206939091e-02]  
 [-4.877301055604123e-02 -2.485186683174640e-02  
 -6.573876335888401e-02 -1.150626323775211e-01  
 -4.279365689880904e-03 -8.158280321388127e-03  
 -2.726480705357713e-02 1.433960674511918e-02  
 1.581557227509544e-02 7.161721353324697e-03  
 1.582532773174946e-02 1.127068678623845e-02]  
 [1.196640196527907e-02 -2.205681711348016e-03  
 -6.561211558325156e-01 -9.898284199745649e-02  
 -4.111900136766620e-02 4.091101962810028e-02  
 -2.574654456174966e-02 -8.000789553709935e-02  
 2.938624353221080e-02 -7.330043946075164e-02  
 -7.501434754208548e-02 2.702115451940091e-02]  
 [-6.076420425957026e-02 2.118765974951407e-02  
 2.790644668306521e-02 4.302423347047137e-02  
 -3.535239959531846e-02 -3.928586149926752e-02  
 -1.125413536441100e-01 4.520249046722492e-02  
 4.057036691535994e-02 9.899090432448526e-02  
 6.769283120563314e-01 -2.440231612349794e-01]  
 [-1.891374455476427e-03 -4.055143024329234e-02  
 -6.950361472612172e-03 -2.509512995738588e-02  
 1.155338214675095e-01 1.495522586119980e-01  
 8.652477212711691e-03 5.310012215519515e-02  
 -1.515067796505897e-01 2.500167075355087e-02  
 1.465810971257825e-02 -9.347770100829896e-02]  
 [3.033754228466455e-02 -5.840828872696023e-03  
 6.819630622079304e-02 1.272581048151417e-02  
 -1.916154197417996e-01 1.110504082209816e-01  
 2.398951012412319e-01 -3.172411143375876e-03  
 5.162092846310068e-02 -5.833365239469306e-04  
 1.082183964422926e-01 3.598062256801164e-01]  
 [6.265020389843116e-02 8.533905051522710e-02  
 -9.778948197972424e-03 7.574275235762509e-02

3.428414065656851e-02 7.797440408903665e-02  
7.934284303764479e-02 2.261937406497748e-02  
-7.693989811698243e-02 -2.832686508657857e-02  
-2.522213072858225e-02 4.421956274607653e-02]  
[4.072899952225332e-02 9.001971876507607e-02  
4.844751603303540e-02 4.977609484628085e-02  
-8.772819918044159e-03 -4.819145761181171e-02  
-1.069845735948595e-01 3.343740287280909e-02  
-8.175395744707950e-02 4.886680642655285e-02  
8.047432191910569e-01 2.351509609240563e-01]

34

[2.361657051689271e-02 -1.544610121741909e-01  
3.506301131211357e-02 -8.241799116745684e-02  
5.874784532947556e-02 -8.520754769671445e-02  
-1.014115145660988e-01 -3.049093740666372e-02  
1.789968170061607e-02 1.897746758260719e-02  
5.616469070248384e-02 5.419620392813455e-04]  
[4.495441762456490e-02 9.175162693743759e-02  
4.982590983644770e-02 4.944596383929024e-02  
-1.561548504692334e-02 -8.884077431628100e-03  
-8.744157514286344e-02 9.300287988611174e-04  
-6.860104922020031e-02 2.251609462529758e-03  
6.937106186536005e-01 2.411317079988303e-01]  
[2.045613771446065e-03 1.238512191939662e-02  
7.392003961095896e-02 3.918041337838498e-02  
8.088811242367163e-04 5.022336746234719e-02  
-1.372845036387844e-03 -1.112097296757984e-01  
-8.154365479455692e-03 3.838707395598631e-02  
1.854338172868382e-01 8.288939849230317e-02]  
[8.092760855556051e-03 -1.076338328339881e-01  
5.980136641918439e-03 -8.621246334070826e-02  
-8.674840803101336e-02 1.950566374115723e-01  
1.806569792312571e-01 6.221523009966079e-02  
2.844789007762647e-02 -1.784070353961133e-02  
-9.322368694782737e-02 6.454991739708074e-02]  
[-3.794287121870312e-03 -3.820534983454497e-02  
-8.098506573351345e-02 -6.532575306883624e-02  
5.113590673008979e-02 -1.469858745590425e-02  
-3.941747565229212e-02 -5.668909099976585e-02  
-4.199643075881419e-02 2.738829204919933e-02  
1.737195296424007e-02 -5.500907251361530e-03]  
[-6.390203416549100e-03 9.148974343033720e-03  
3.054920061720997e-02 2.963384039449136e-02  
-9.515006931287827e-02 4.547595300280526e-03  
2.199476452690874e-01 -4.907335759205765e-03  
4.328728298346131e-02 8.616378939032254e-02  
7.527981370675193e-01 5.592883514637337e-01]  
[-9.048918975546993e-02 -5.231410726653411e-02  
-8.475213626793990e-02 -1.978578883841151e-02

8.490745394252037e-01 1.385791533664747e-01  
 5.238370684465738e-02 9.576180566469904e-02  
 1.021934264366295e-02 -3.775052422399468e-02  
 8.554663769737602e-03 9.164884002607715e-02]  
 [8.026149026055759e-02 4.623551183905958e-02  
 7.130734689586657e-03 5.694641535347757e-02  
 1.077771544279737e-01 1.873336795899415e-01  
 3.587046352755727e-02 1.430743536588534e-02  
 -2.037181836870995e-01 -7.758111557374678e-02  
 -8.643569165980977e-02 1.147829232252137e-02]  
 [1.197625810361132e-02 -2.234524124941284e-03  
 -6.561068886784408e-01 -9.870456759359310e-02  
 -4.121065302387163e-02 4.082965752097371e-02  
 -2.562331543841764e-02 -8.003467753976543e-02  
 2.953540452870769e-02 -7.325988337366654e-02  
 -7.509886834823475e-02 2.686965414062156e-02]  
 [-7.567627616177676e-02 3.316672872172647e-03  
 1.904432875866055e-02 4.404111146216842e-02  
 -2.893977238102160e-02 5.835793833822297e-03  
 -2.850630676258084e-02 9.115081019853846e-02  
 3.369795675133391e-02 2.399926484256683e-02  
 1.609305855135884e-01 -4.300613989652821e-01]  
 [-1.881533015677825e-01 1.120331662877659e-01  
 -1.436200118876921e-01 3.805751562118359e-02  
 1.918777016645180e-03 -3.326727380400489e-03  
 -7.186106197672367e-03 2.612795618226559e-03  
 3.489797777474292e-03 1.420176881096530e-03  
 -2.765050509303815e-03 2.228746086788584e-03]

35

[-9.097879271083474e-02 -5.437285485086259e-02  
 -8.746824529292570e-02 -2.363118719960296e-02  
 8.373709331202582e-01 6.368559814373306e-02  
 9.030323156180597e-02 7.167685943239545e-02  
 -4.372171591246735e-03 -6.584967268041901e-02  
 4.923986128148358e-02 9.926697452460029e-02]  
 [1.190220975539262e-02 -2.230898848179745e-03  
 -6.561279517556374e-01 -9.912449269494532e-02  
 -4.105694762644593e-02 4.099022274632422e-02  
 -2.568093531569409e-02 -8.012170341271543e-02  
 2.931569324892997e-02 -7.333384863232252e-02  
 -7.501554309119220e-02 2.704840259485912e-02]  
 [3.877590179209139e-02 8.859160421908287e-02  
 4.872168536538465e-02 4.888727390440310e-02  
 -3.582820518449423e-02 -5.146786668508794e-03  
 -4.906438356266071e-02 5.378806029527209e-02  
 -1.033672762230429e-01 2.445173817554327e-02  
 8.681409030370922e-01 2.491508074876789e-01]  
 [-4.109772111465508e-02 -8.158350945147772e-02  
 -1.934844251803718e-02 -8.059077433305280e-02]

-1.926537739644273e-02 1.149248305606158e-01  
 3.240403419625931e-02 6.867518343533216e-02  
 7.073105722963017e-03 5.710504021950452e-02  
 -1.075434497235682e-01 2.609759403297376e-02]  
 [7.763771336394036e-02 5.880616150213566e-03  
 1.177822512781298e-01 2.835492286905893e-02  
 -1.810941869364247e-02 1.344485831288592e-02  
 3.577404761975726e-02 -3.301142530193618e-02  
 -2.702825540954001e-03 2.749359134507295e-02  
 2.334454093662311e-02 4.105544150618731e-02]  
 [6.849507304830271e-02 5.339162581963549e-02  
 -8.665715438100935e-03 4.950704199978565e-02  
 1.517297347181984e-01 9.915835302077208e-02  
 3.784231373356335e-02 1.579839904309016e-02  
 -1.870068727778907e-01 3.330332062254510e-02  
 -7.012777508289016e-02 8.046959602490705e-02]  
 [-5.709993976981120e-02 2.280638002121794e-02  
 -6.210906056077128e-02 -4.966108483422844e-02  
 1.530300009262190e-02 -1.766027243341670e-02  
 -4.500752695344541e-02 2.289878194203959e-02  
 1.215987270535990e-02 3.555605832709403e-02  
 -7.875083203582704e-03 2.978843932053393e-02]  
 [-5.827199732507060e-02 2.665287930832242e-02  
 3.164975083601651e-02 4.368485372855812e-02  
 -4.308735930774354e-02 -1.309631420137875e-03  
 -7.387930837720834e-02 1.466352216829195e-02  
 1.100640442816698e-02 7.541217422301963e-02  
 7.255738356118138e-01 -8.468368762532093e-02]  
 [4.732267138554257e-02 -1.942689517959069e-02  
 2.345801587277400e-02 2.132510090466149e-02  
 -1.376879231405265e-01 1.776722796066927e-01  
 2.127637070695595e-01 -3.148627519331580e-02  
 8.204180953456745e-02 -1.384137083846521e-01  
 1.574459513727551e-01 6.173095142795098e-02]  
 [-1.581026373571081e-02 -1.112610644399395e-01  
 2.817735891581388e-02 -3.346226563617164e-02  
 9.243009111955887e-02 2.452988820331137e-02  
 -1.755416228255203e-02 -1.192347353540889e-01  
 -4.043813615129679e-05 1.643064124939202e-02  
 5.425801386596760e-02 1.151399742315370e-01]  
 [-1.462134269712492e-02 3.354924134717348e-01  
 -2.289848103419306e+00 4.790538716497041e-01  
 1.885565741194053e-07 -3.955515069607120e-07  
 -1.361613138879809e-06 -3.326896928696679e-07  
 2.594661139518337e-08 1.129885112911338e-07  
 -8.651167066458035e-08 7.022468690473963e-08]

36

[-4.906431631940556e-02 -9.787547730542576e-02  
 1.693524824401704e-02 -1.043526866261623e-01



2.956710681917683e-03 6.832695404897603e-02  
 3.494752035955048e-02 -3.590466080703778e-02  
 -2.769365355818387e-02 3.859366171278976e-02  
 -6.427362783605493e-02 4.402343630796349e-02]  
 [1.195526458126401e-02 -2.225233107326864e-03  
 -6.560617911550294e-01 -9.889555950767143e-02  
 -4.116236126009046e-02 4.091836657836043e-02  
 -2.569765009158126e-02 -8.005871495073363e-02  
 2.942903883394041e-02 -7.332443870321742e-02  
 -7.507355132817820e-02 2.698526716511838e-02]  
 [9.788283908286220e-02 6.804304565654817e-02  
 -7.882905769910584e-03 7.784682290777489e-02  
 -6.087676971147429e-02 1.565188843708339e-02  
 2.267652603563135e-03 7.624758003105854e-02  
 2.181115975199975e-02 -4.523388208311416e-02  
 -1.941221848105892e-02 -1.772496328596922e-04]  
 [-2.551245435177232e-02 -1.016694263393545e-01  
 2.666877958863974e-02 -2.021985137029832e-02  
 5.191302374190113e-02 2.939387668007784e-02  
 2.407511176737645e-02 -6.812814731485987e-02  
 -1.506997666324321e-03 1.870339052400754e-02  
 -2.395677777317357e-02 1.223577102052945e-01]  
 [-9.145190185003320e-02 -5.246161372501253e-02  
 -8.783837535852630e-02 -2.164876604774241e-02  
 8.091322130470857e-01 1.006262524032847e-01  
 7.774023874575672e-02 8.587146905038354e-02  
 -9.171204590532455e-04 -6.572677575034024e-02  
 4.925667128839906e-02 9.324226635401703e-02]  
 [9.469776211766751e-02 2.682540413855243e-02  
 6.006436066271486e-03 5.210162961088844e-02  
 1.526800263891437e-01 1.688961161341570e-01  
 9.224003855986823e-02 -1.490905612548004e-01  
 -1.755333442521667e-01 -2.903165588476605e-02  
 1.541180216362805e-02 -1.310926765407586e-02]  
 [-5.671599135545249e-02 3.073231792856122e-02  
 3.240508869918560e-02 4.415838725797368e-02  
 -5.161169267840097e-02 -3.196992264532694e-02  
 -1.039207449922907e-01 3.023474830663968e-02  
 5.549117071792634e-03 8.491520910730244e-02  
 7.572715115533862e-01 1.466004679723008e-02]  
 [7.576646449142956e-02 6.927741571111851e-02  
 2.318028307004189e-02 5.806905832448752e-02  
 1.391923220088792e-02 6.391012315307620e-02  
 7.361074162766260e-02 5.175727023046425e-02  
 -7.684115410816424e-02 -2.111997573978111e-02  
 -2.946411021860518e-02 1.390732757907074e-01]  
 [3.228543432228827e-02 8.856907049413752e-02  
 4.953215244148454e-02 4.854068846558993e-02  
 -6.171398143248230e-02 -4.047118577804566e-02  
 -1.011595644786203e-01 1.120006790500652e-01

-7.697518633250049e-02 3.867873550175588e-02  
8.585105826279736e-01 6.205925446329534e-02]  
[-3.315894902872397e-02 -5.623762150531790e-02  
-7.029844371972099e-03 -9.531101058472692e-02  
1.643316522166771e-02 5.546944768475492e-04  
-6.835104927045709e-03 8.294944015124364e-02  
1.028320847168877e-01 1.509572448557320e-02  
5.025993427199701e-02 5.248731152741093e-02]  
[5.136174008566098e-02 2.184883207673759e-02  
7.726739373447913e-02 3.858563811449411e-02  
-2.987084994223955e-02 9.445178103227467e-02  
1.306314169020064e-01 -1.222327681277510e-01  
4.395338331908533e-02 3.060545428307932e-02  
9.891095222451844e-02 1.034625124264928e-01]

*E-mail address:* elena.angelini@unisi.it
